# Supplementary material for: Implicit Hari--Zimmermann algorithm for the generalized SVD on the GPUs
Source: arXiv:1909.00101 ancillary file (2020-10-13)
Supplement: Supplementary file 1 [file sm.pdf]

Journal Title
XX(X):1–93
©The Author(s) 2020
Reprints and permission:
sagepub.co.uk/journalsPermissions.nav
DOI: 10.1177/ToBeAssigned
www.sagepub.com/
SAGE

# Supplementary material for the "Implicit Hari–Zimmermann algorithm for the generalized SVD on the GPUs" manuscript

**Vedran Novaković[1] and Sanja Singer[2]**

**Abstract**

This is a supplementary material accompanying the paper "Implicit Hari–Zimmermann algorithm for the generalized SVD on the GPUs", comprising two sections (to be regarded as appendices), inclusion of which in the paper would be impractical. However, understanding of some aspects of the Hari–Zimmermann algorithm and its behavior might be enhanced by this material and therefore it would be beneficial to make it available alongside the paper itself.

**Keywords**

parallel pivot strategies, numerical testing results

In section 1 two continuous animations of the parallel Jacobi strategies, one for ME and one for MM, are shown for the matrix order $n = 32$. *Adobe Acrobat Reader is recommended for running the animations*!

In section 2 the numerical testing results on the small dataset are shown for all single-GPU variants of the real and the complex Hari–Zimmermann algorithm. The captions of the figures included therein should be self-explanatory. The real portion of the small dataset is available at:
`http://euridika.math.hr:1846/Jacobi/FLdata/GPU/D/`
and the complex portion of the small and the large datasets is available at:
`http://euridika.math.hr:1846/Jacobi/FLdata/GPU/Z/`
URLs. The `xz`-compressed files contain only the binary stored matrices $F$ (`Y`) and $G$ (`W`), in double (complex) datatype and in the Fortran array order.

[1]Completed a major part of this research while being affiliated to Universidad Jaime I, Av. Vicent Sos Baynat, 12071 Castellón de la Plana, Spain
[2]University of Zagreb, Faculty of Mechanical Engineering and Naval Architecture, Ivana Lučića 5, 10000 Zagreb, Croatia

**Corresponding author:**
Sanja Singer, University of Zagreb, Faculty of Mechanical Engineering and Naval Architecture, Ivana Lučića 5, 10000 Zagreb, Croatia
Email: ssinger@fsb.hr

Please refer to `https://github.com/venovako/GPUHZGSVD` repository for the source code implementation of the algorithm in CUDA C++ (and MPI for the multi-GPU).

Finally, the reader is encouraged to take a look at a pixel-per-element animation of a run of the full block (`00`) and the block-oriented (`08`) ZHZ0 algorithm variant on a matrix of order $n = 512$, *viewed two-sidedly*, at
`http://euridika.math.hr:1846/Jacobi/FLdata/GPU/ZHZ-0/` or
`https://github.com/venovako/GPUHZGSVD/tree/master/ZHZ-0` URLs.

## 1 Parallel pivot strategies

Figures 1 and 2 show continuous animations of the Mantharam–Eberlein (ME) Mantharam and Eberlein (1993) parallel Jacobi cyclic strategy, and the modified modulus (MM) Novaković and Singer (2011); Novaković et al. (2015)) quasi-cyclic strategy, respectively, on a matrix of order 32. The former strategy with the same matrix order is used for the innermost level of the Hari–Zimmermann algorithm, i.e., for the pointwise algorithm on the shared memory within a GPU.

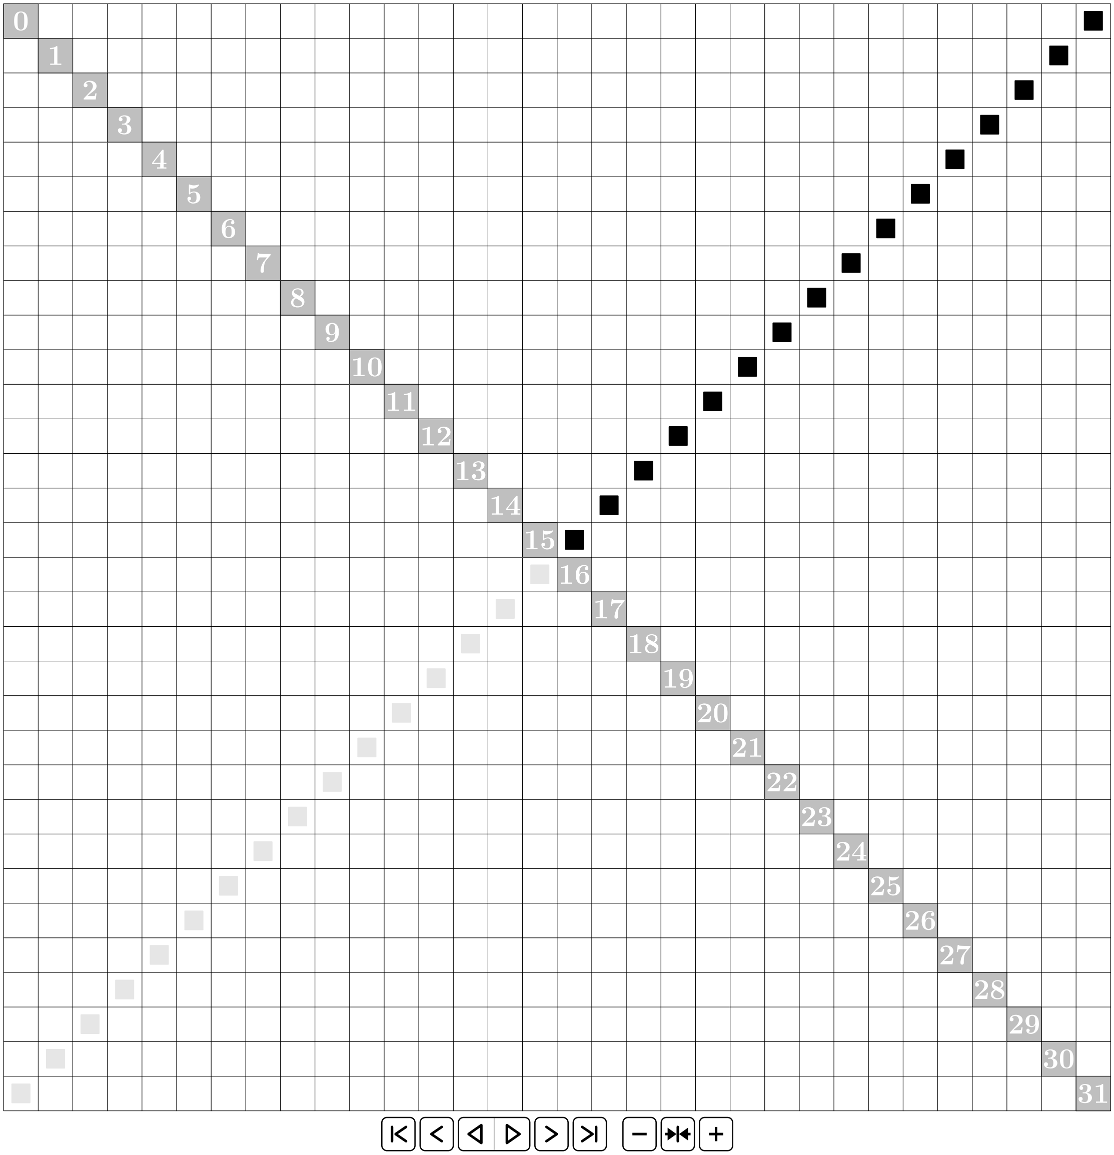


**Figure 1.** A step-by-step illustration of the ME (Mantharam–Eberlein) parallel Jacobi cyclic strategy, on a matrix of order $32$. Viewed two-sidedly, in each parallel step, a black square and its grayed reflection across the diagonal represent a pivot pair to be annihilated (i.e., a pair of columns to be orthogonalized one-sidedly). Together with the corresponding diagonal elements, those $4$ elements in total form a $2 \times 2$ pivot submatrix from which a Jacobi rotation is to be computed. After $31$ steps, the annihilation sequence is repeated, i.e., a fresh cycle (sweep) starts if the convergence criterion has not been satisfied. The row/column indices, $0$-based, are shown on the diagonal.

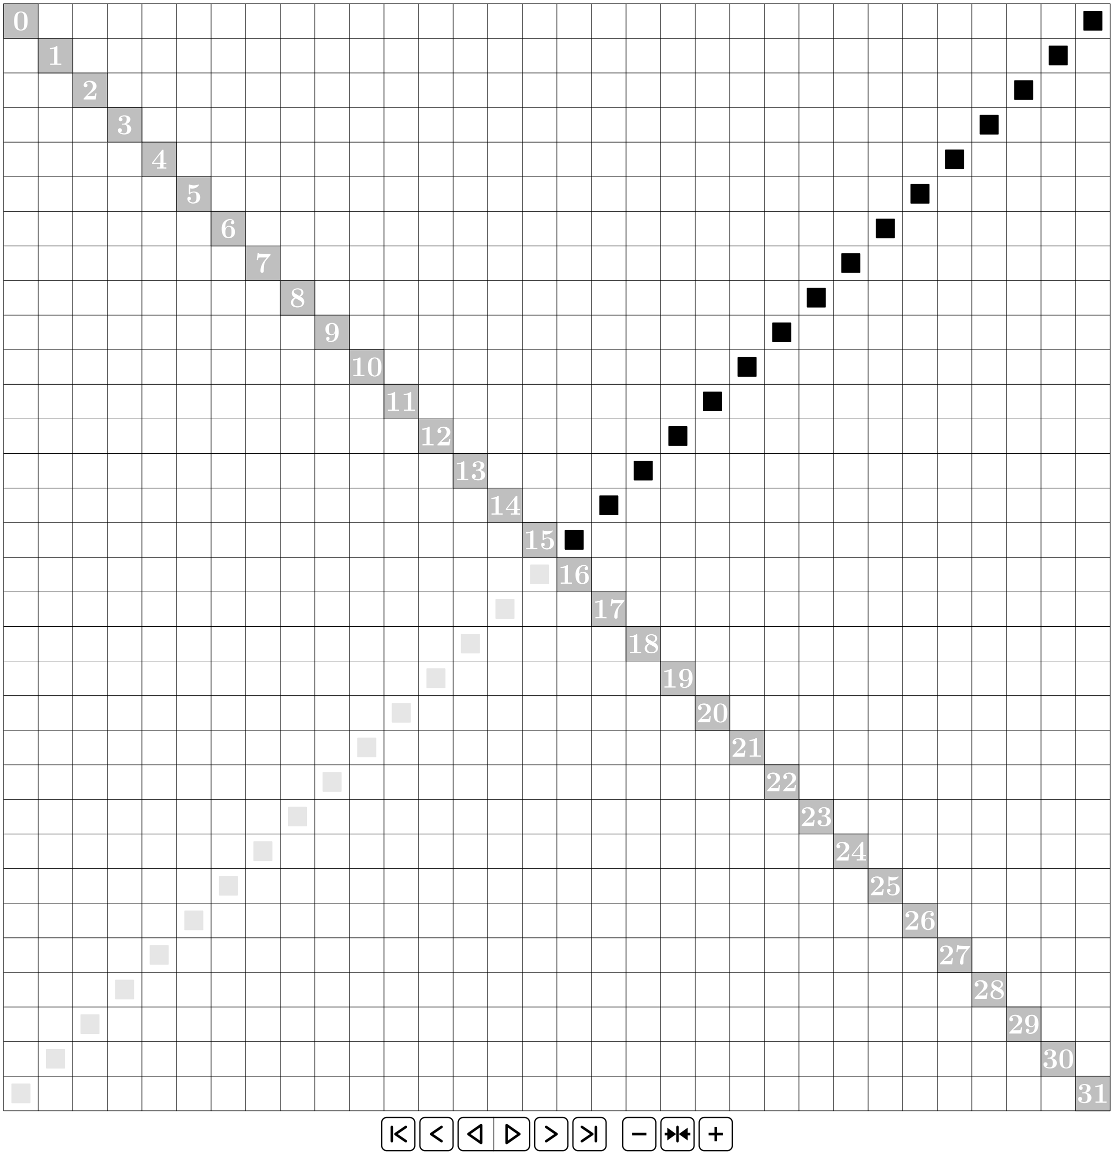


**Figure 2.** A step-by-step illustration of the MM (modified modulus) parallel Jacobi **quasi**-cyclic strategy, on a matrix of order $32$. Viewed two-sidedly, in each parallel step, a black square and its grayed reflection across the diagonal represent a pivot pair to be annihilated (i.e., a pair of columns to be orthogonalized one-sidedly). Together with the corresponding diagonal elements, those $4$ elements in total form a $2 \times 2$ pivot submatrix from which a Jacobi rotation is to be computed. After $\mathbf{32}$ steps, where a total of $16$ pivot pairs are annihilated twice (one in each odd step, counting from $0$), the annihilation sequence is repeated, i.e., a fresh cycle (sweep) starts if the convergence criterion has not been satisfied. The row/column indices, $0$-based, are shown on the diagonal.

# 2 Numerical testing results (single-GPU)

## *2.1 DHZ*

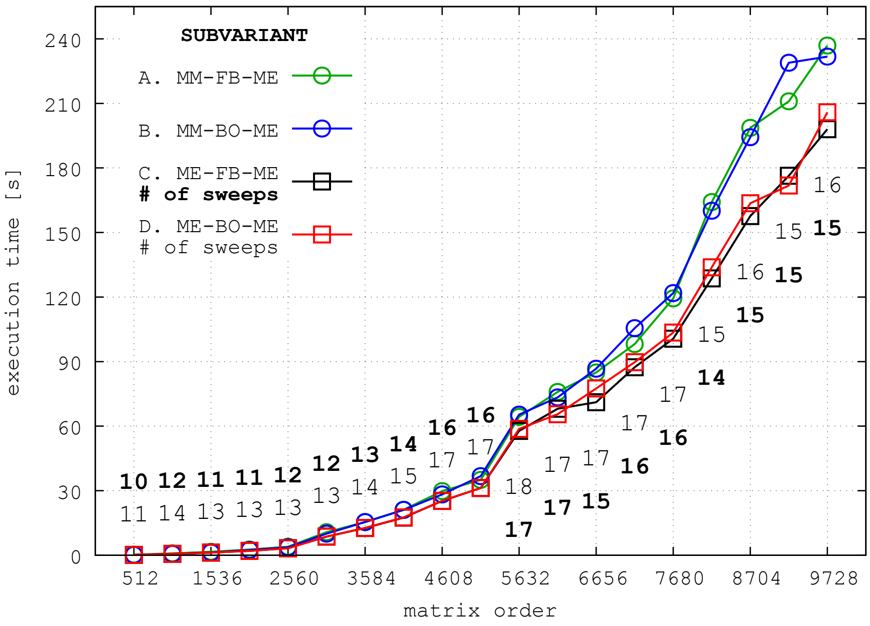


**Figure 3.** The wall execution time and the number of block sweeps for the the block-oriented (BO) and the full block (FB) DHZ variants, with the outer Jacobi strategies chosen as ME or MM (the inner strategy always being ME), for the Algorithm **DHZ0** and the matrices from the test set, with orders varying from $512$ to $9728$. The number of sweeps is shown for the ME-BO and the ME-FB (in **bold**). For the MM strategy those numbers are usually larger than for the corresponding ME-using variant.

### *2.1.1 DHZ0*

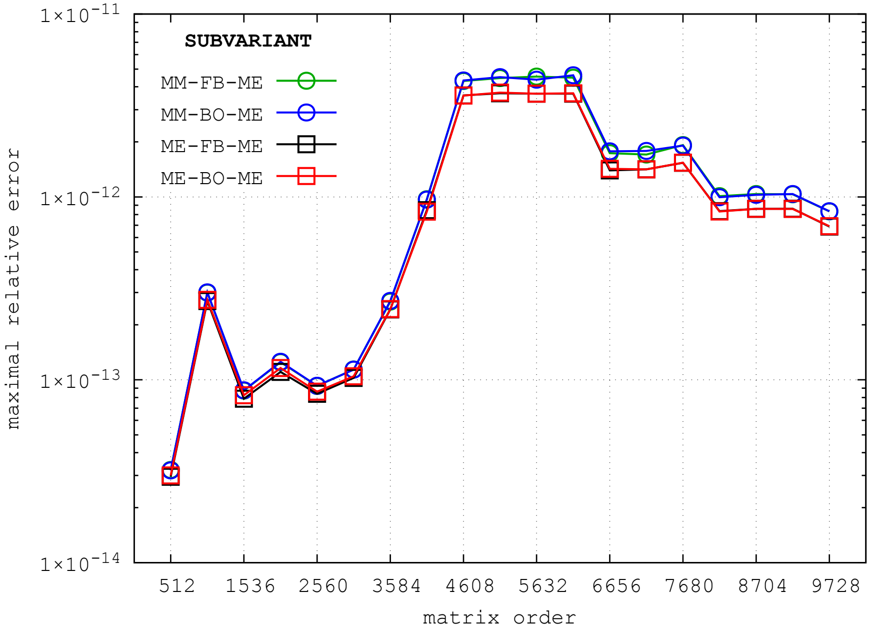


**Figure 4.** The maximal normwise relative error in the computed decomposition of the first matrix in a matrix pair, $\|F - U\Sigma_F X\|_F / \|F\|_F$, for the Algorithm **DHZ0** on the matrices from the test set, with orders varying from $512$ to $9728$.

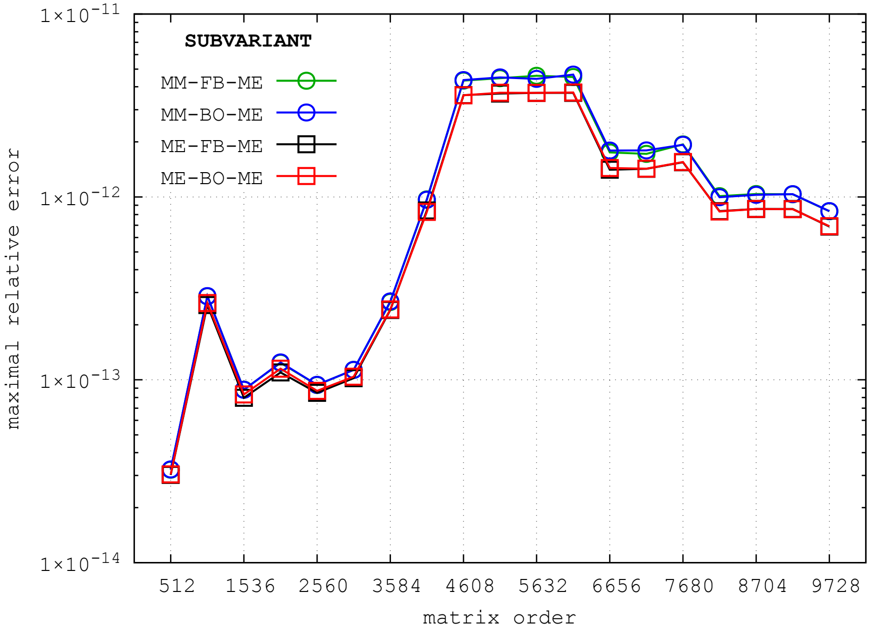


**Figure 5.** The maximal normwise relative error in the computed decomposition of the second matrix in a matrix pair, $\|G - V\Sigma_G X\|_F / \|G\|_F$, for the Algorithm **DHZ0** on the matrices from the test set, with orders varying from $512$ to $9728$.

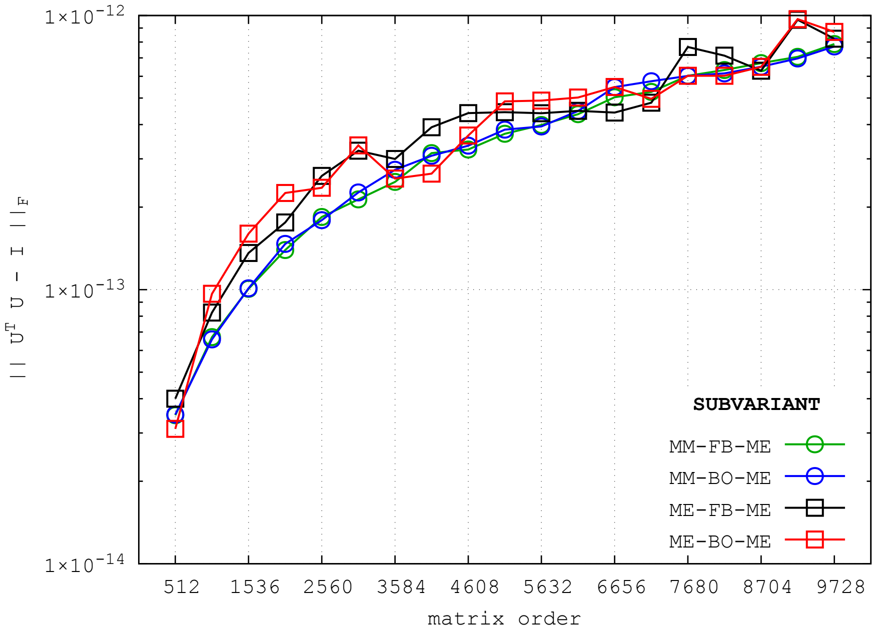


**Figure 6.** Orthogonality $\|U^T U - I\|_F$ of the left generalized singular vectors $U$ for the Algorithm **DHZ0** on the matrices from the test set, with orders varying from $512$ to $9728$.

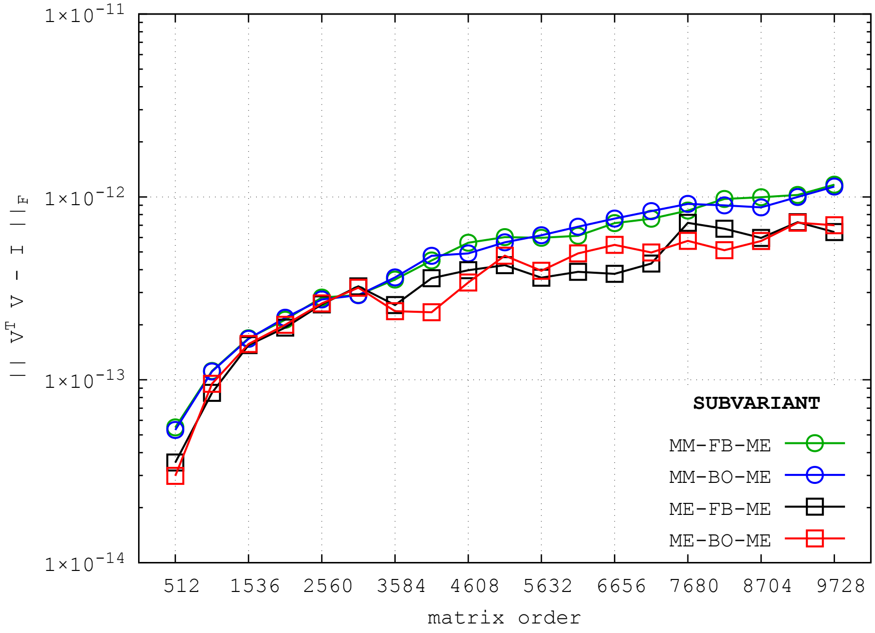


**Figure 7.** Orthogonality $\|V^T V - I\|_F$ of the left generalized singular vectors $V$ for the Algorithm **DHZ0** on the matrices from the test set, with orders varying from $512$ to $9728$.

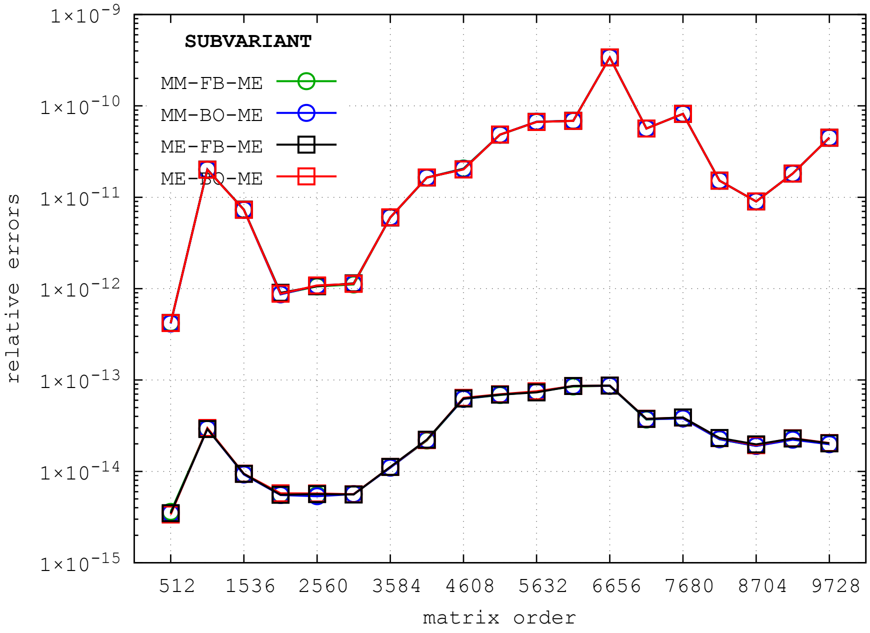


**Figure 8.** The maximal (upper graph) and the average (lower graph) relative errors in the computed versus the original generalized singular values for the Algorithm **DHZ0** on the matrices from the test set, with orders varying from $512$ to $9728$. Neither the choice of a DHZ variant, nor of an outer Jacobi strategy, affects the errors much in those test cases.

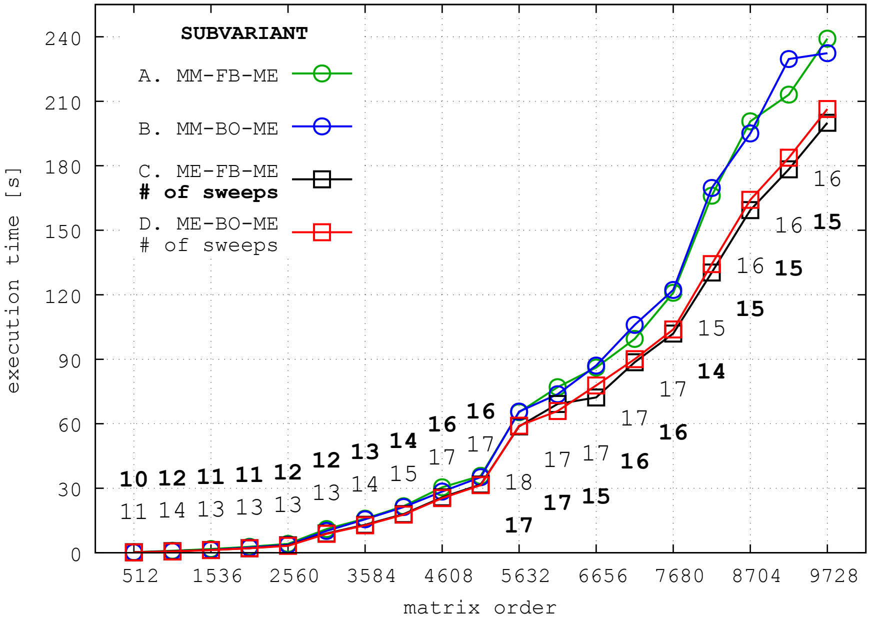


**Figure 9.** The wall execution time and the number of block sweeps for the the block-oriented (BO) and the full block (FB) DHZ variants, with the outer Jacobi strategies chosen as ME or MM (the inner strategy always being ME), for the Algorithm **DHZ1** and the matrices from the test set, with orders varying from $512$ to $9728$. The number of sweeps is shown for the ME-BO and the ME-FB (in **bold**). For the MM strategy those numbers are usually larger than for the corresponding ME-using variant.

### *2.1.2 DHZ1*

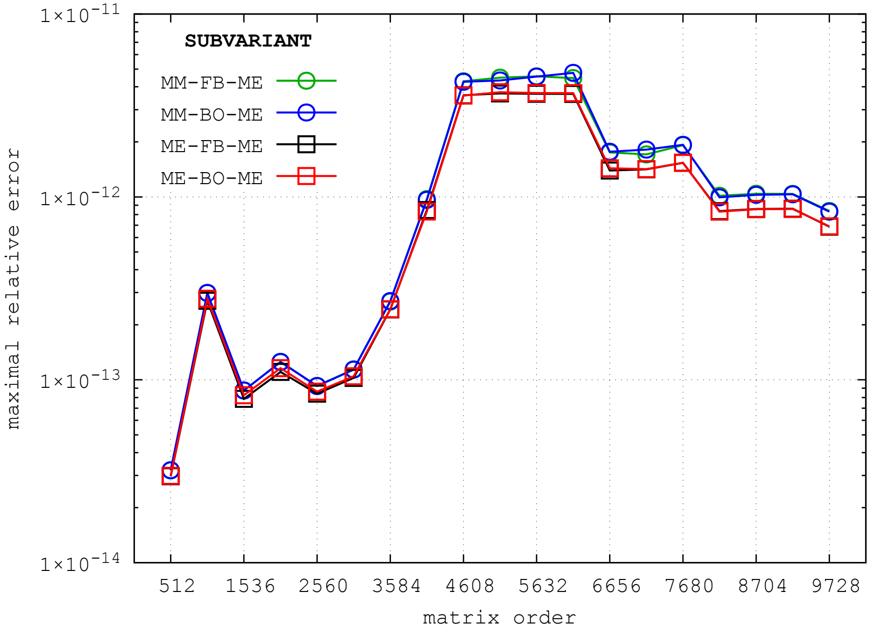


**Figure 10.** The maximal normwise relative error in the computed decomposition of the first matrix in a matrix pair, $\|F - U\Sigma_F X\|_F / \|F\|_F$, for the Algorithm **DHZ1** on the matrices from the test set, with orders varying from $512$ to $9728$.

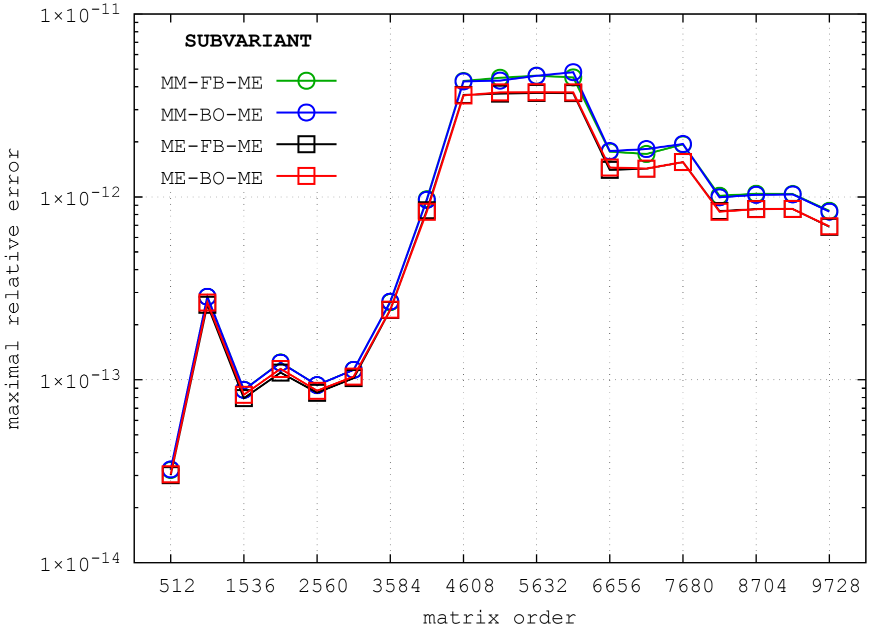


**Figure 11.** The maximal normwise relative error in the computed decomposition of the second matrix in a matrix pair, $\|G - V\Sigma_G X\|_F/\|G\|_F$, for the Algorithm **DHZ1** on the matrices from the test set, with orders varying from $512$ to $9728$.

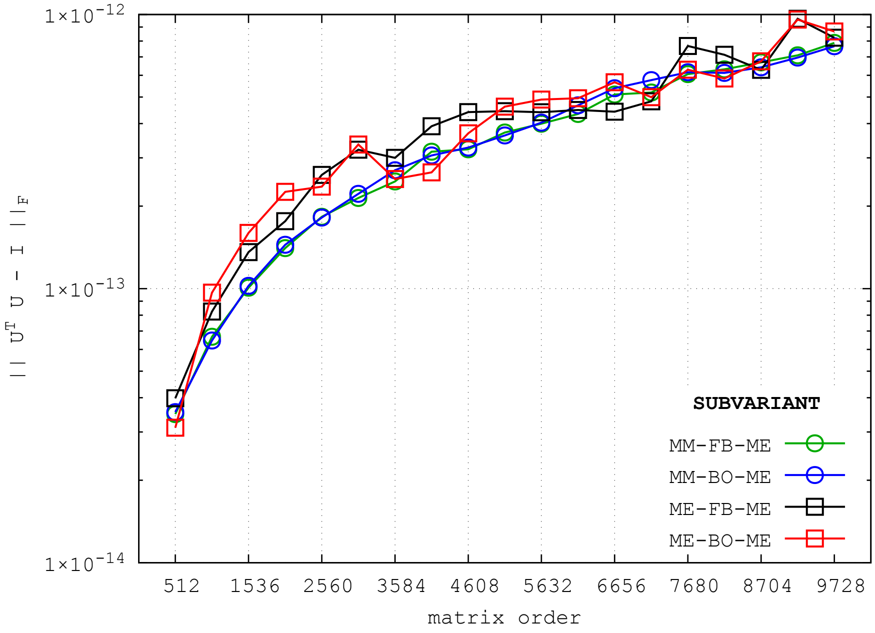


**Figure 12.** Orthogonality $\|U^T U - I\|_F$ of the left generalized singular vectors $U$ for the Algorithm **DHZ1** on the matrices from the test set, with orders varying from $512$ to $9728$.

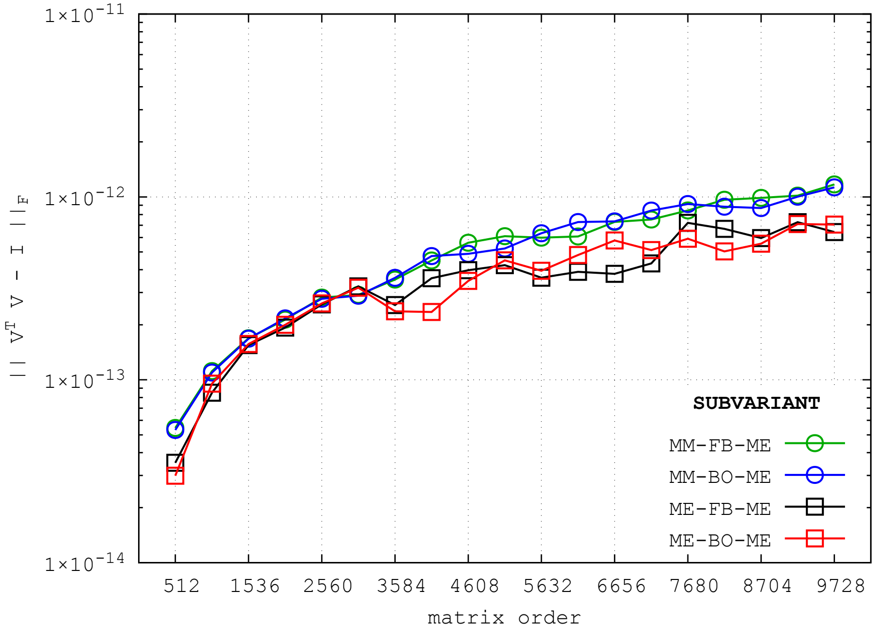


**Figure 13.** Orthogonality $\|V^T V - I\|_F$ of the left generalized singular vectors $V$ for the Algorithm **DHZ1** on the matrices from the test set, with orders varying from $512$ to $9728$.

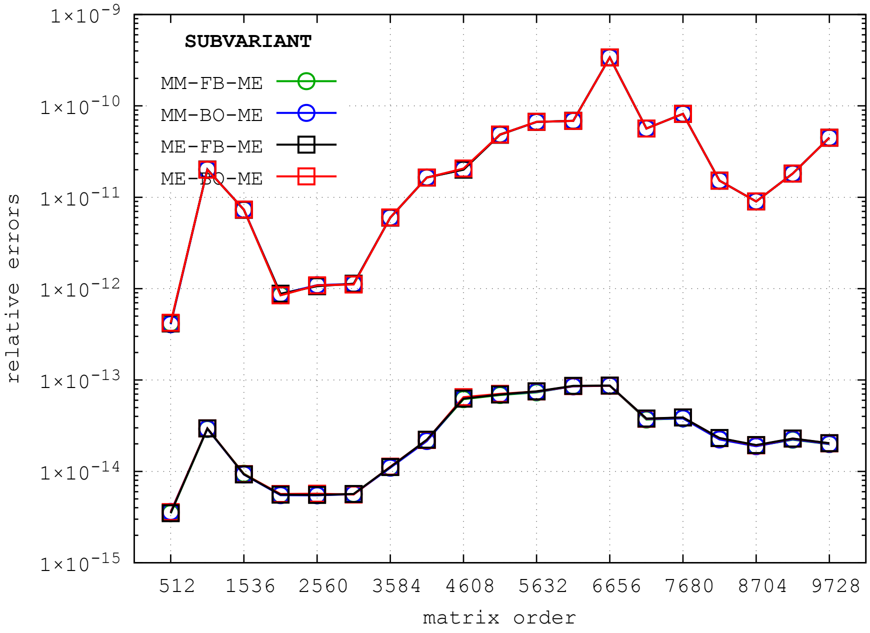


**Figure 14.** The maximal (upper graph) and the average (lower graph) relative errors in the computed versus the original generalized singular values for the Algorithm **DHZ1** on the matrices from the test set, with orders varying from $512$ to $9728$. Neither the choice of a DHZ variant, nor of an outer Jacobi strategy, affects the errors much in those test cases.

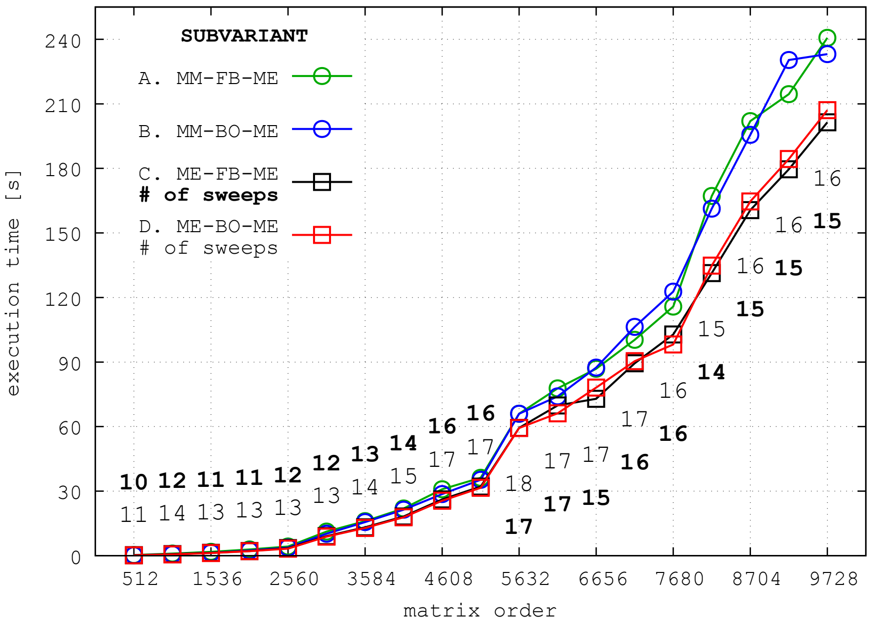


**Figure 15.** The wall execution time and the number of block sweeps for the the block-oriented (BO) and the full block (FB) DHZ variants, with the outer Jacobi strategies chosen as ME or MM (the inner strategy always being ME), for the Algorithm **DHZ2** and the matrices from the test set, with orders varying from $512$ to $9728$. The number of sweeps is shown for the ME-BO and the ME-FB (in **bold**). For the MM strategy those numbers are usually larger than for the corresponding ME-using variant.

### *2.1.3 DHZ2*

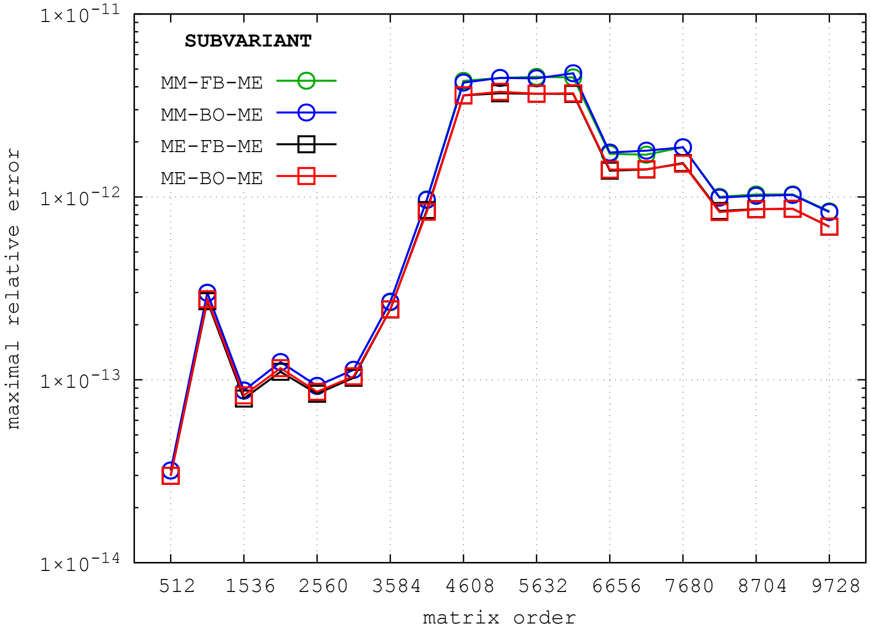


**Figure 16.** The maximal normwise relative error in the computed decomposition of the first matrix in a matrix pair, $\|F - U\Sigma_F X\|_F / \|F\|_F$, for the Algorithm **DHZ2** on the matrices from the test set, with orders varying from $512$ to $9728$.

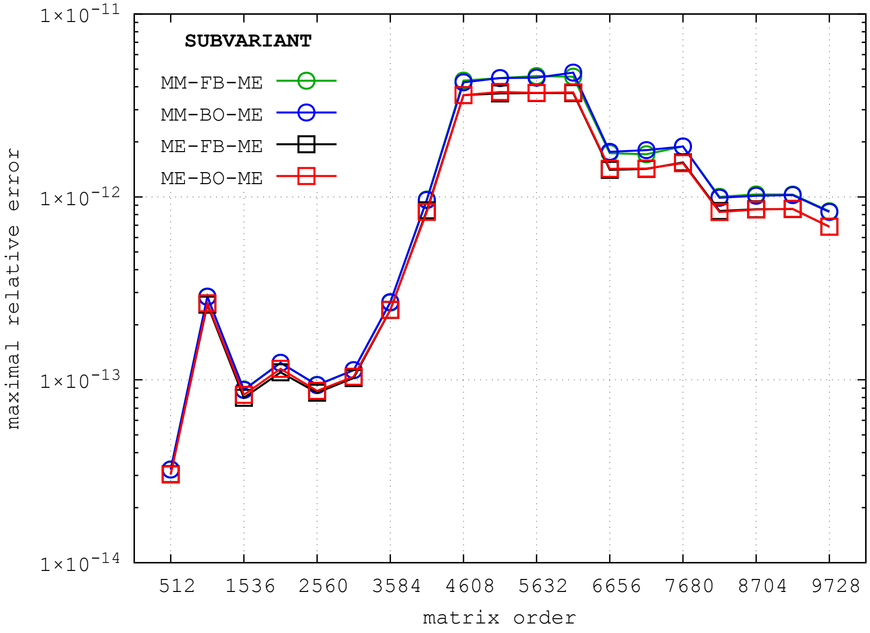


**Figure 17.** The maximal normwise relative error in the computed decomposition of the second matrix in a matrix pair, $\|G - V\Sigma_G X\|_F / \|G\|_F$, for the Algorithm **DHZ2** on the matrices from the test set, with orders varying from $512$ to $9728$.

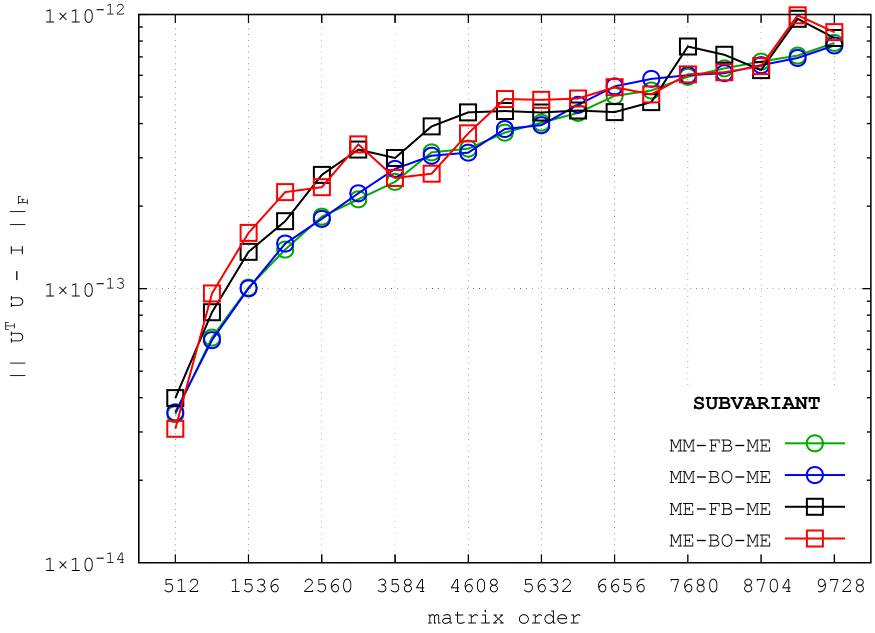


**Figure 18.** Orthogonality $\|U^T U - I\|_F$ of the left generalized singular vectors $U$ for the Algorithm **DHZ2** on the matrices from the test set, with orders varying from $512$ to $9728$.

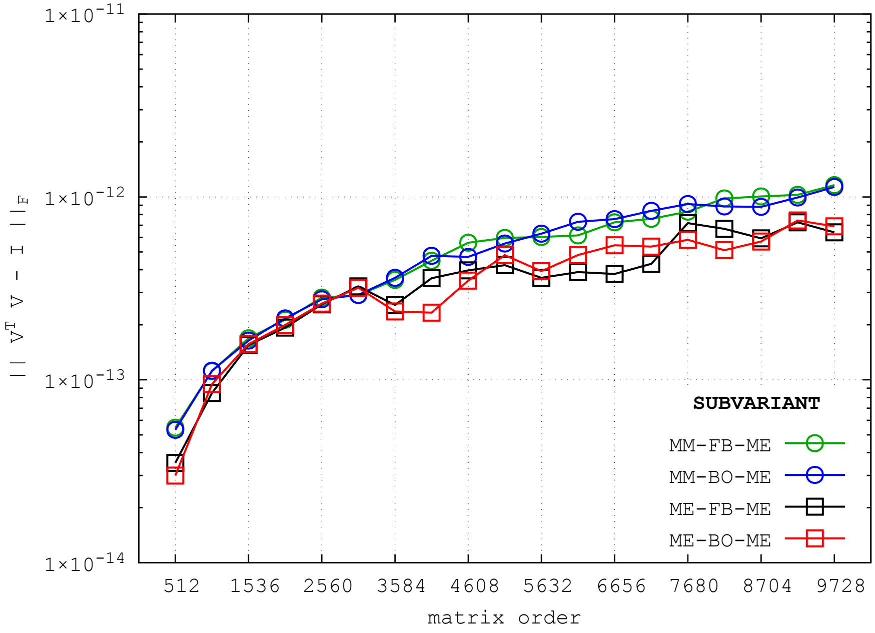


**Figure 19.** Orthogonality $\|V^T V - I\|_F$ of the left generalized singular vectors $V$ for the Algorithm **DHZ2** on the matrices from the test set, with orders varying from $512$ to $9728$.

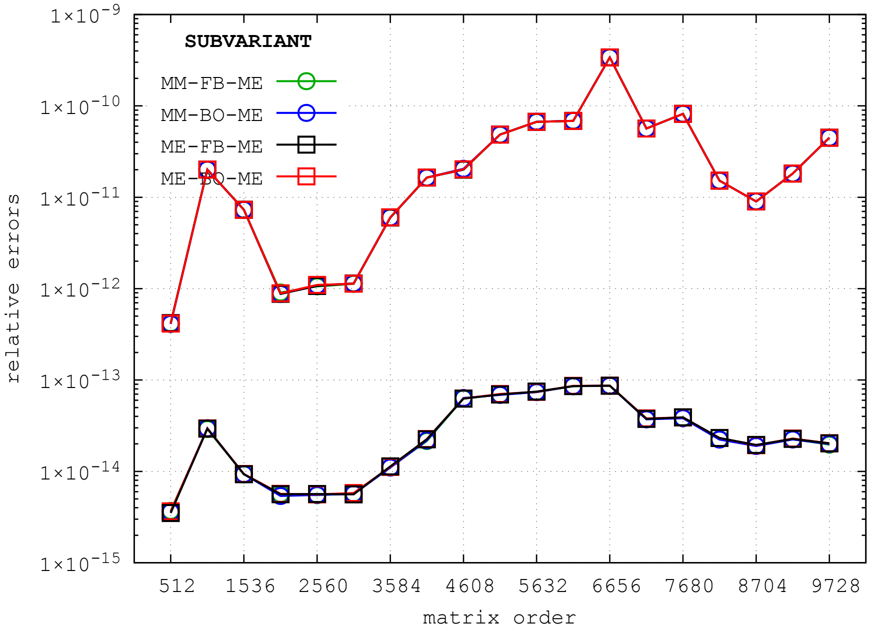


**Figure 20.** The maximal (upper graph) and the average (lower graph) relative errors in the computed versus the original generalized singular values for the Algorithm **DHZ2** on the matrices from the test set, with orders varying from $512$ to $9728$. Neither the choice of a DHZ variant, nor of an outer Jacobi strategy, affects the errors much in those test cases.

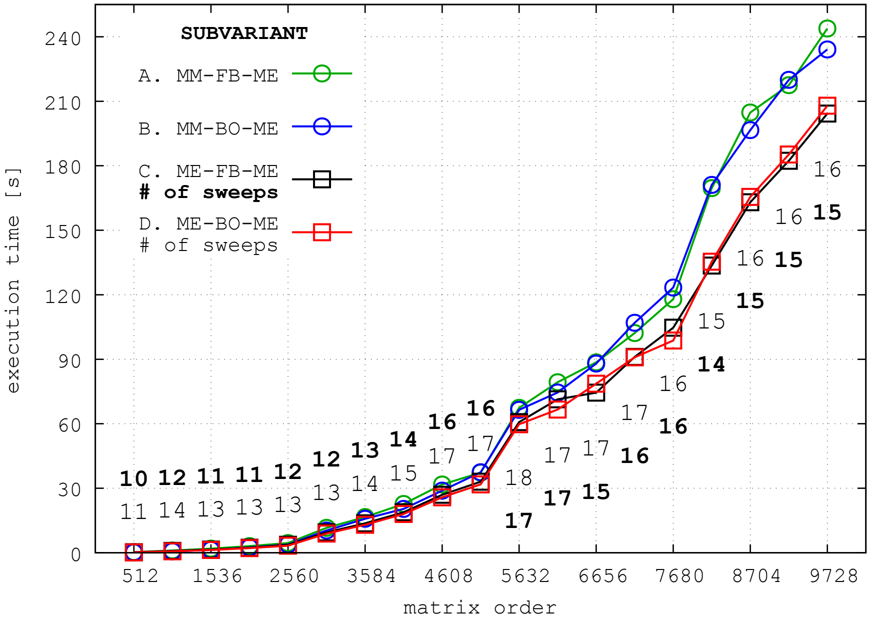


**Figure 21.** The wall execution time and the number of block sweeps for the the block-oriented (BO) and the full block (FB) DHZ variants, with the outer Jacobi strategies chosen as ME or MM (the inner strategy always being ME), for the Algorithm **DHZ3** and the matrices from the test set, with orders varying from $512$ to $9728$. The number of sweeps is shown for the ME-BO and the ME-FB (in **bold**). For the MM strategy those numbers are usually larger than for the corresponding ME-using variant.

### *2.1.4 DHZ3*

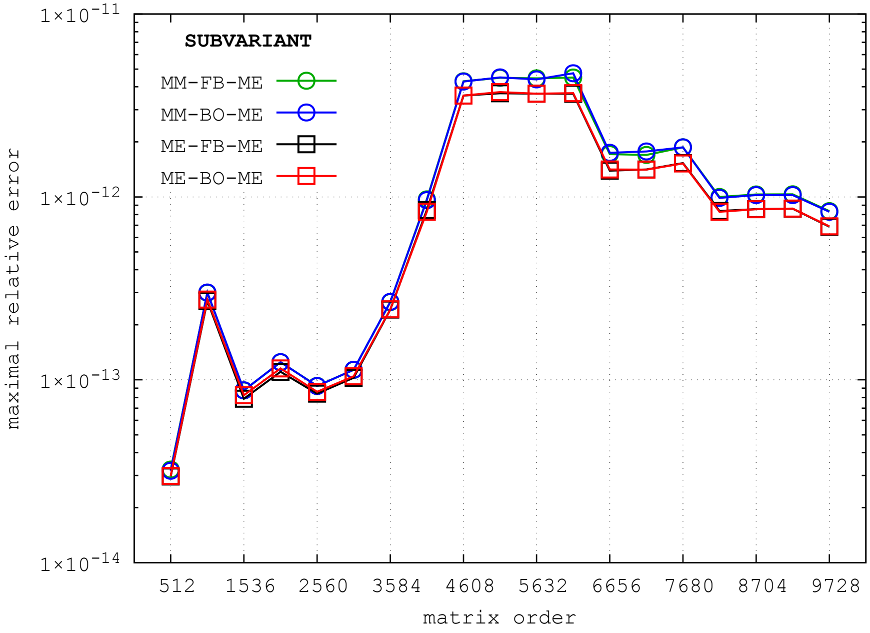


**Figure 22.** The maximal normwise relative error in the computed decomposition of the first matrix in a matrix pair, $\|F - U\Sigma_F X\|_F / \|F\|_F$, for the Algorithm **DHZ3** on the matrices from the test set, with orders varying from $512$ to $9728$.

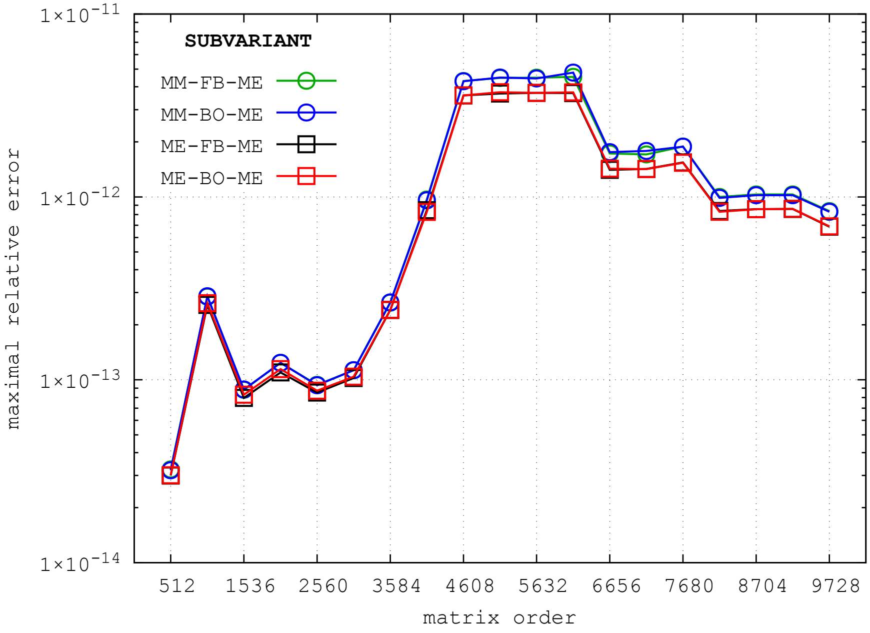


**Figure 23.** The maximal normwise relative error in the computed decomposition of the second matrix in a matrix pair, $\|G - V\Sigma_G X\|_F / \|G\|_F$, for the Algorithm **DHZ3** on the matrices from the test set, with orders varying from $512$ to $9728$.

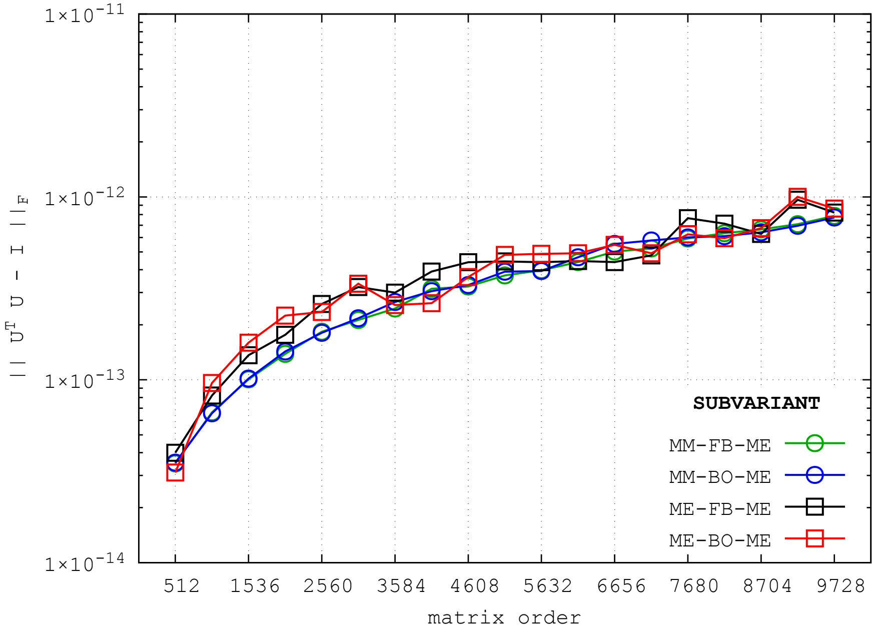


**Figure 24.** Orthogonality $\|U^T U - I\|_F$ of the left generalized singular vectors $U$ for the Algorithm **DHZ3** on the matrices from the test set, with orders varying from $512$ to $9728$.

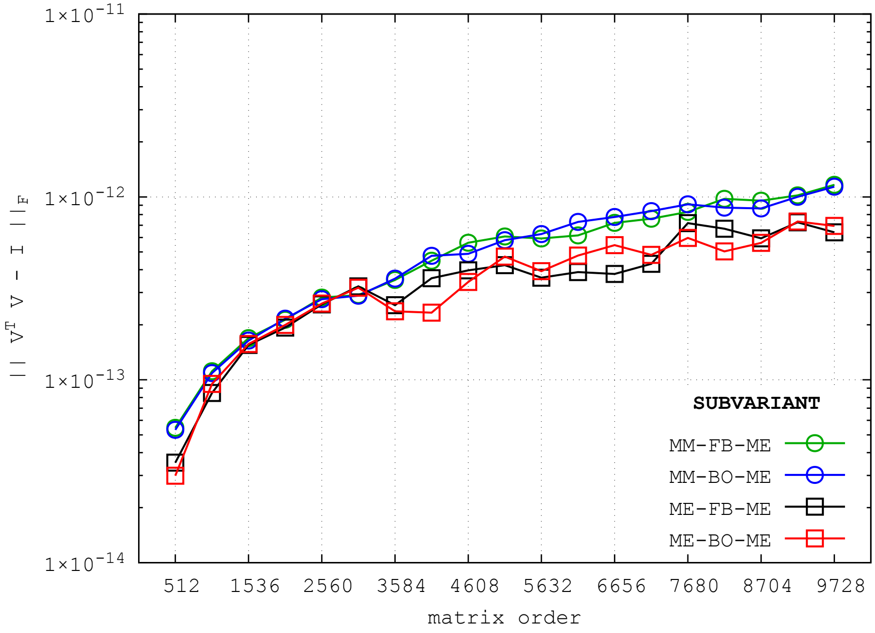


**Figure 25.** Orthogonality $\|V^T V - I\|_F$ of the left generalized singular vectors $V$ for the Algorithm **DHZ3** on the matrices from the test set, with orders varying from $512$ to $9728$.

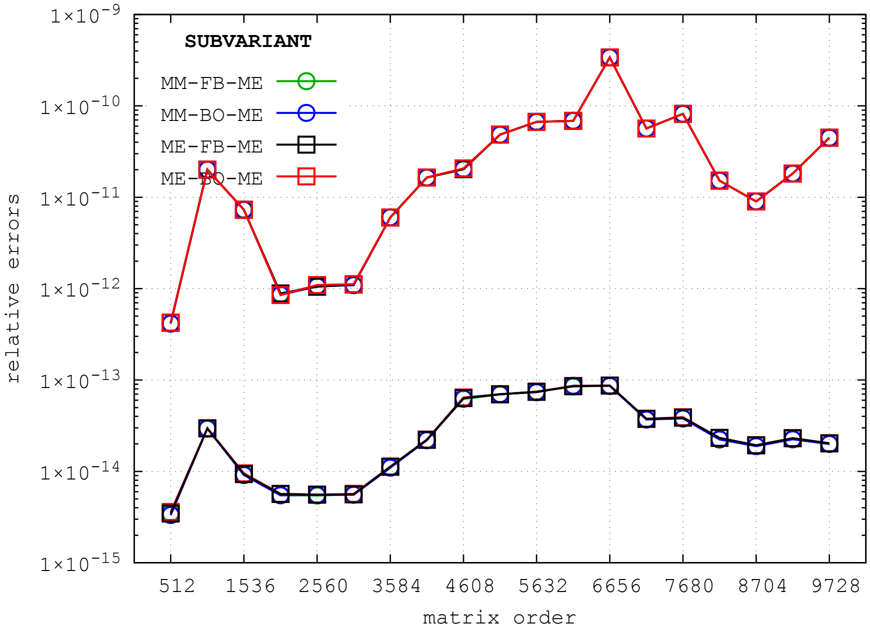


**Figure 26.** The maximal (upper graph) and the average (lower graph) relative errors in the computed versus the original generalized singular values for the Algorithm **DHZ3** on the matrices from the test set, with orders varying from $512$ to $9728$. Neither the choice of a DHZ variant, nor of an outer Jacobi strategy, affects the errors much in those test cases.

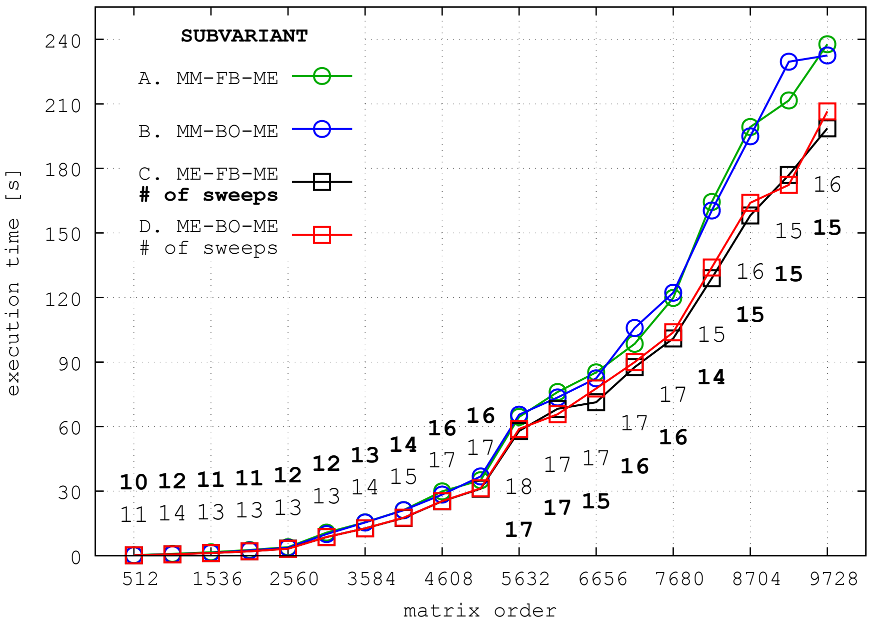


**Figure 27.** The wall execution time and the number of block sweeps for the the block-oriented (BO) and the full block (FB) DHZ variants, with the outer Jacobi strategies chosen as ME or MM (the inner strategy always being ME), for the Algorithm **DHZ4** and the matrices from the test set, with orders varying from $512$ to $9728$. The number of sweeps is shown for the ME-BO and the ME-FB (in **bold**). For the MM strategy those numbers are usually larger than for the corresponding ME-using variant.

### 2.1.5 *DHZ4*

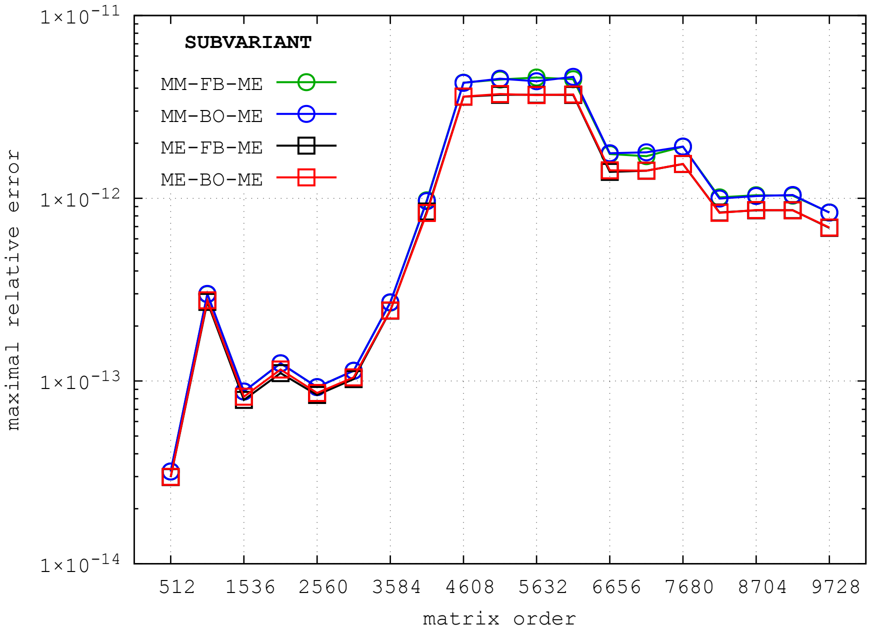


**Figure 28.** The maximal normwise relative error in the computed decomposition of the first matrix in a matrix pair, $\|F - U\Sigma_F X\|_F / \|F\|_F$, for the Algorithm **DHZ4** on the matrices from the test set, with orders varying from $512$ to $9728$.

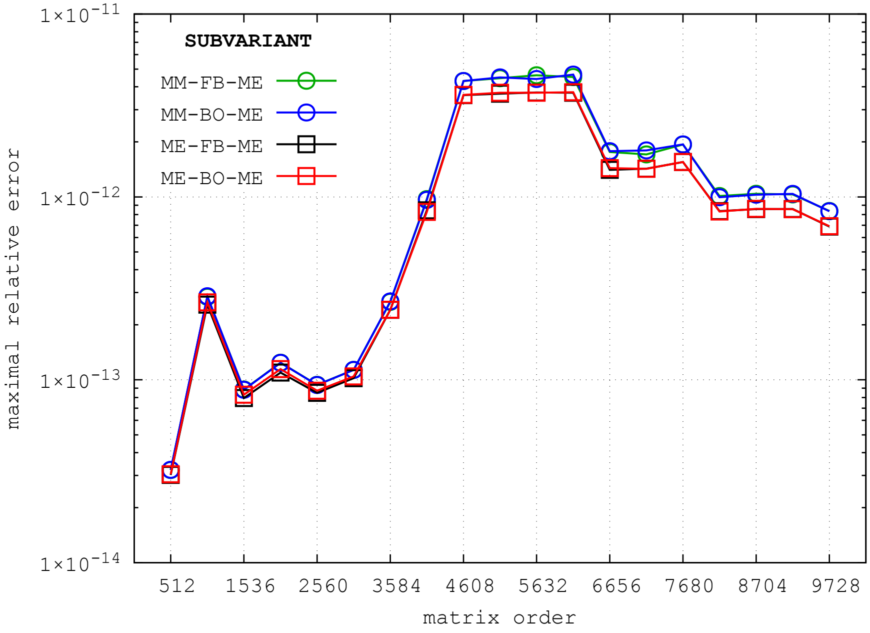


**Figure 29.** The maximal normwise relative error in the computed decomposition of the second matrix in a matrix pair, $\|G - V\Sigma_G X\|_F/\|G\|_F$, for the Algorithm **DHZ4** on the matrices from the test set, with orders varying from $512$ to $9728$.

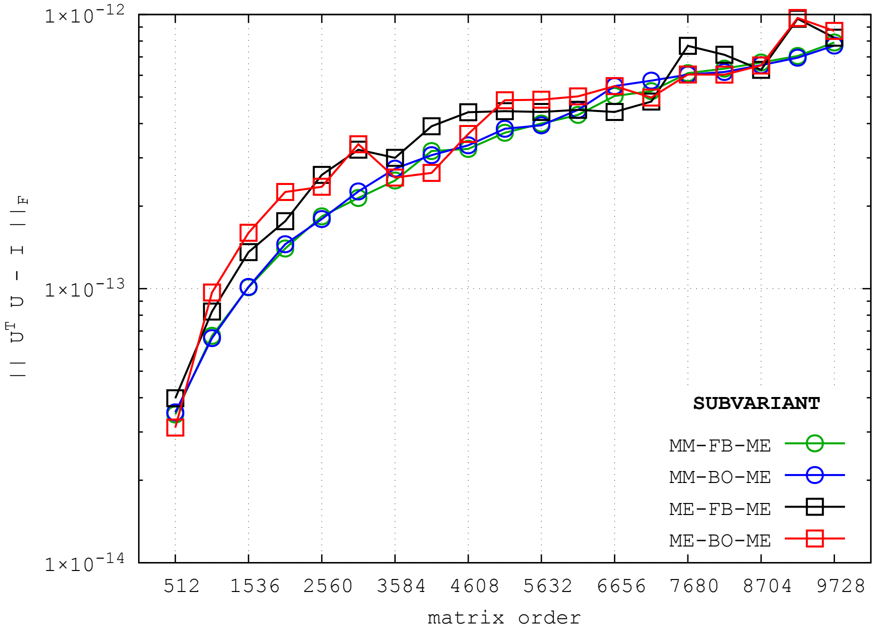


**Figure 30.** Orthogonality $\|U^T U - I\|_F$ of the left generalized singular vectors $U$ for the Algorithm **DHZ4** on the matrices from the test set, with orders varying from $512$ to $9728$.

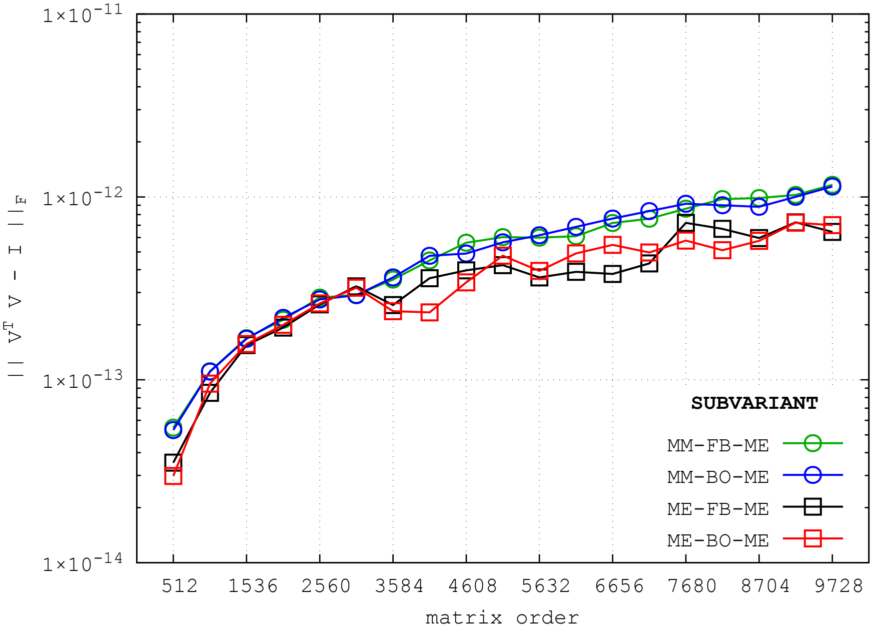


**Figure 31.** Orthogonality $\|V^T V - I\|_F$ of the left generalized singular vectors $V$ for the Algorithm **DHZ4** on the matrices from the test set, with orders varying from $512$ to $9728$.

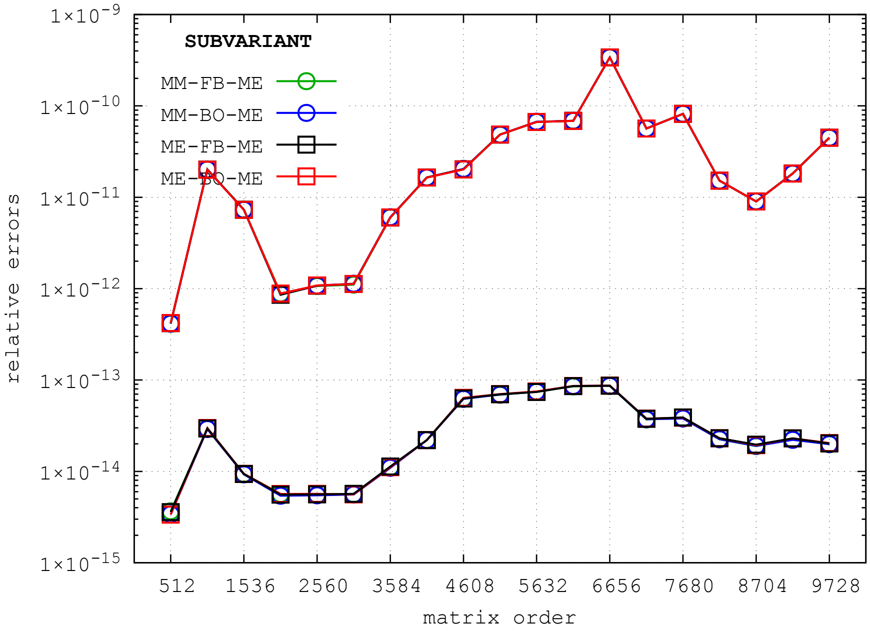


**Figure 32.** The maximal (upper graph) and the average (lower graph) relative errors in the computed versus the original generalized singular values for the Algorithm **DHZ4** on the matrices from the test set, with orders varying from $512$ to $9728$. Neither the choice of a DHZ variant, nor of an outer Jacobi strategy, affects the errors much in those test cases.

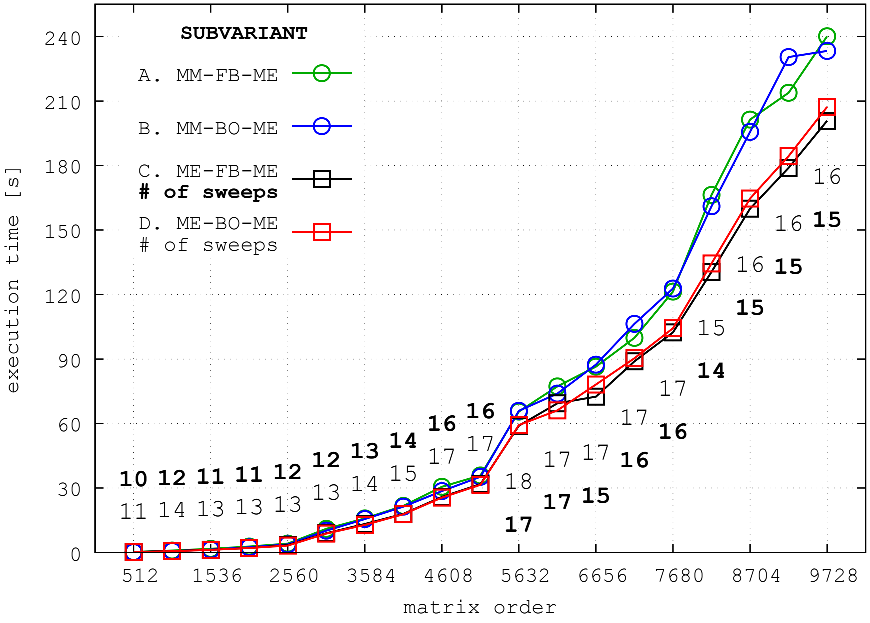


**Figure 33.** The wall execution time and the number of block sweeps for the the block-oriented (BO) and the full block (FB) DHZ variants, with the outer Jacobi strategies chosen as ME or MM (the inner strategy always being ME), for the Algorithm **DHZ5** and the matrices from the test set, with orders varying from $512$ to $9728$. The number of sweeps is shown for the ME-BO and the ME-FB (in **bold**). For the MM strategy those numbers are usually larger than for the corresponding ME-using variant.

### *2.1.6 DHZ5*

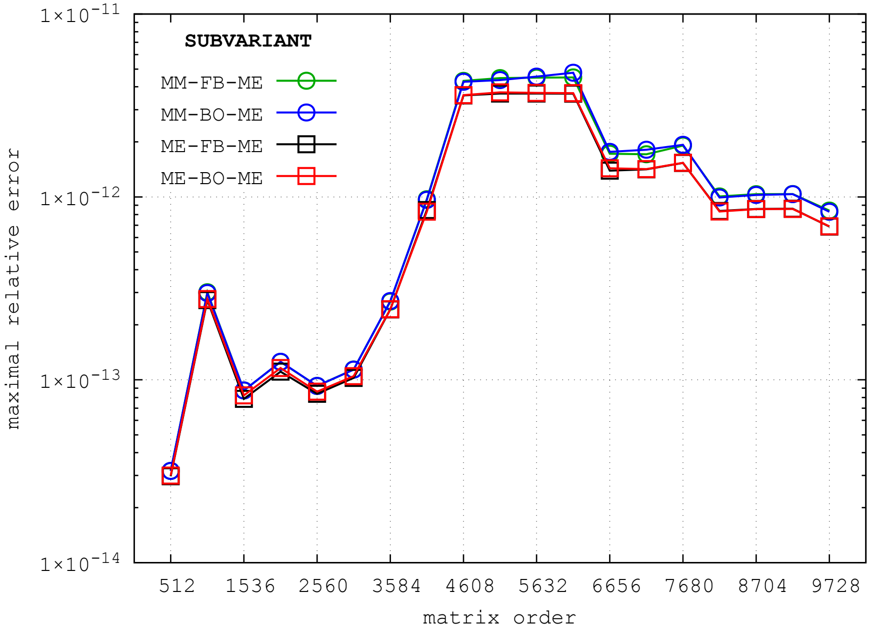


**Figure 34.** The maximal normwise relative error in the computed decomposition of the first matrix in a matrix pair, $\|F - U\Sigma_F X\|_F / \|F\|_F$, for the Algorithm **DHZ5** on the matrices from the test set, with orders varying from $512$ to $9728$.

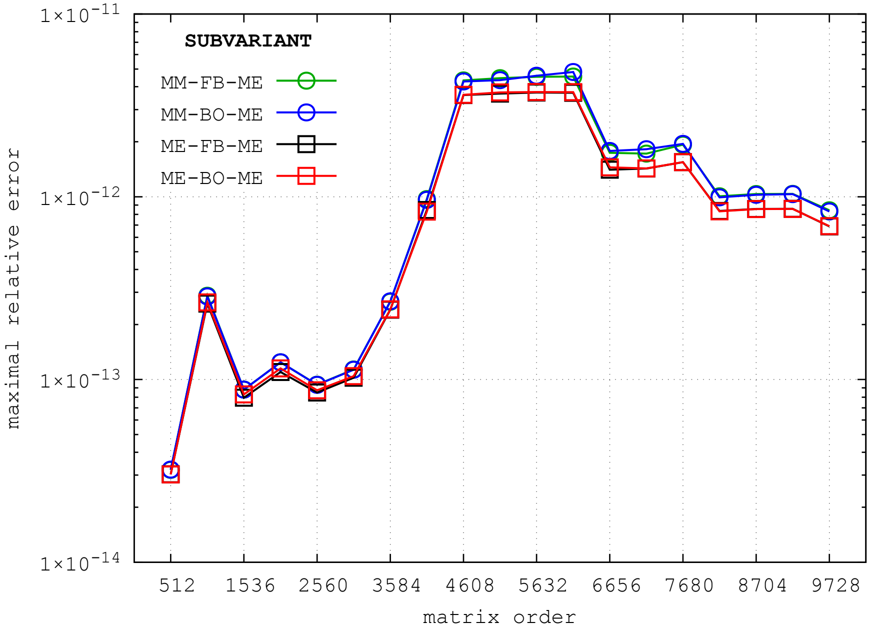


**Figure 35.** The maximal normwise relative error in the computed decomposition of the second matrix in a matrix pair, $\|G - V\Sigma_G X\|_F / \|G\|_F$, for the Algorithm **DHZ5** on the matrices from the test set, with orders varying from $512$ to $9728$.

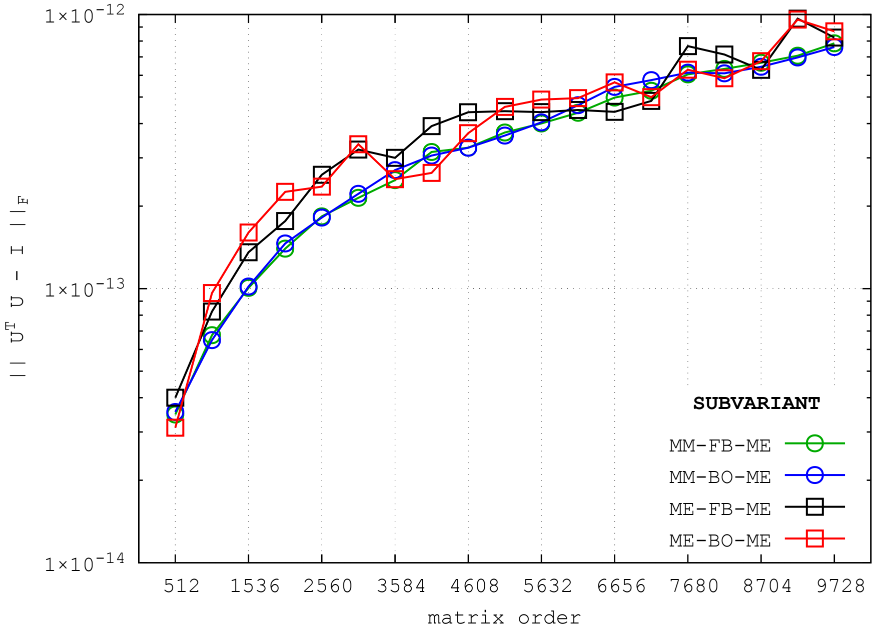


**Figure 36.** Orthogonality $\|U^T U - I\|_F$ of the left generalized singular vectors $U$ for the Algorithm **DHZ5** on the matrices from the test set, with orders varying from $512$ to $9728$.

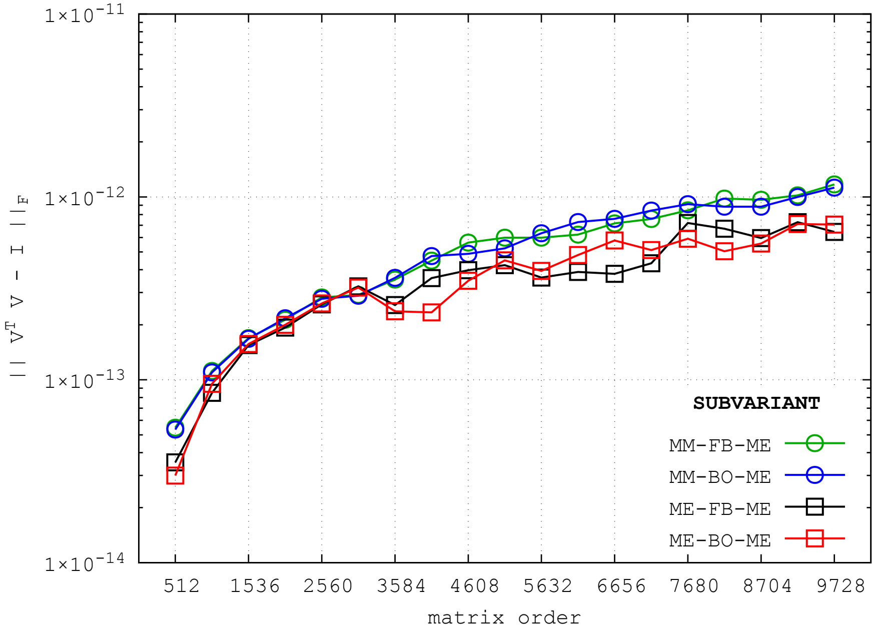


**Figure 37.** Orthogonality $\|V^T V - I\|_F$ of the left generalized singular vectors $V$ for the Algorithm **DHZ5** on the matrices from the test set, with orders varying from $512$ to $9728$.

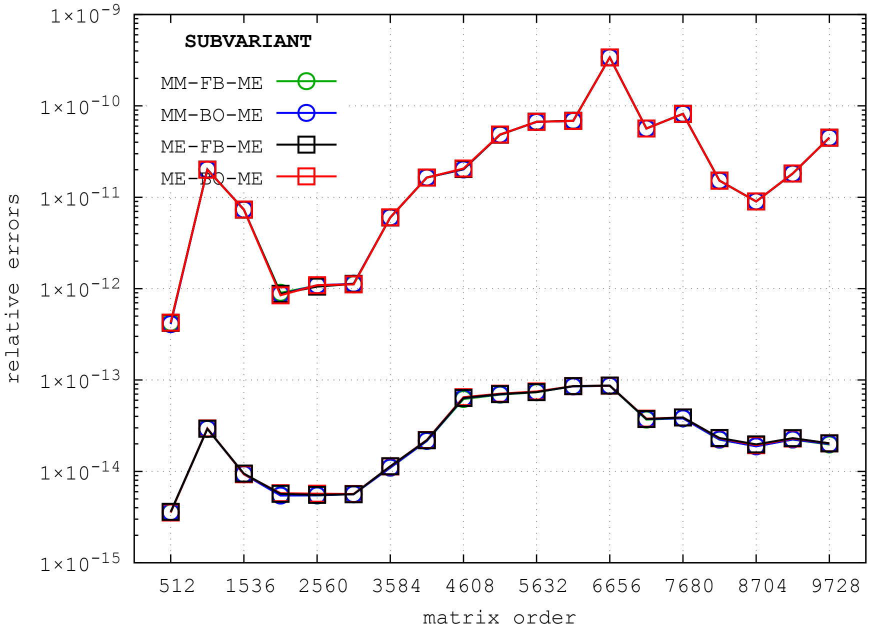


**Figure 38.** The maximal (upper graph) and the average (lower graph) relative errors in the computed versus the original generalized singular values for the Algorithm **DHZ5** on the matrices from the test set, with orders varying from $512$ to $9728$. Neither the choice of a DHZ variant, nor of an outer Jacobi strategy, affects the errors much in those test cases.

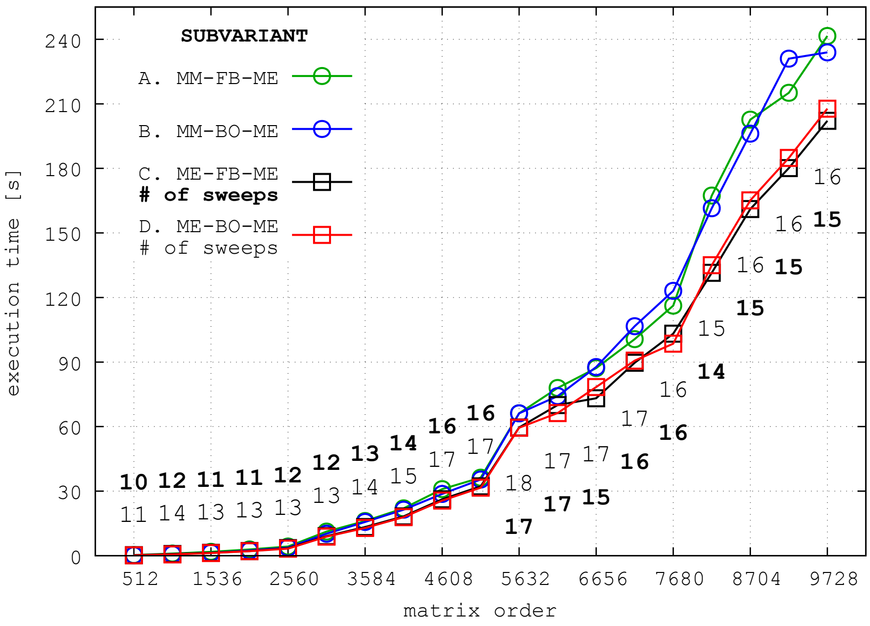


**Figure 39.** The wall execution time and the number of block sweeps for the the block-oriented (BO) and the full block (FB) DHZ variants, with the outer Jacobi strategies chosen as ME or MM (the inner strategy always being ME), for the Algorithm **DHZ6** and the matrices from the test set, with orders varying from $512$ to $9728$. The number of sweeps is shown for the ME-BO and the ME-FB (in **bold**). For the MM strategy those numbers are usually larger than for the corresponding ME-using variant.

### *2.1.7 DHZ6*

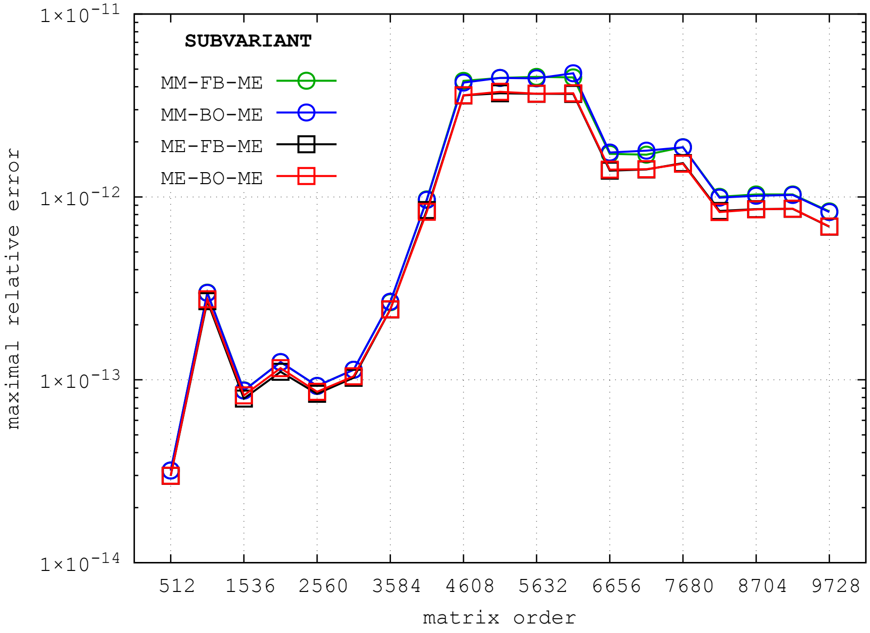


**Figure 40.** The maximal normwise relative error in the computed decomposition of the first matrix in a matrix pair, $\|F - U\Sigma_F X\|_F / \|F\|_F$, for the Algorithm **DHZ6** on the matrices from the test set, with orders varying from $512$ to $9728$.

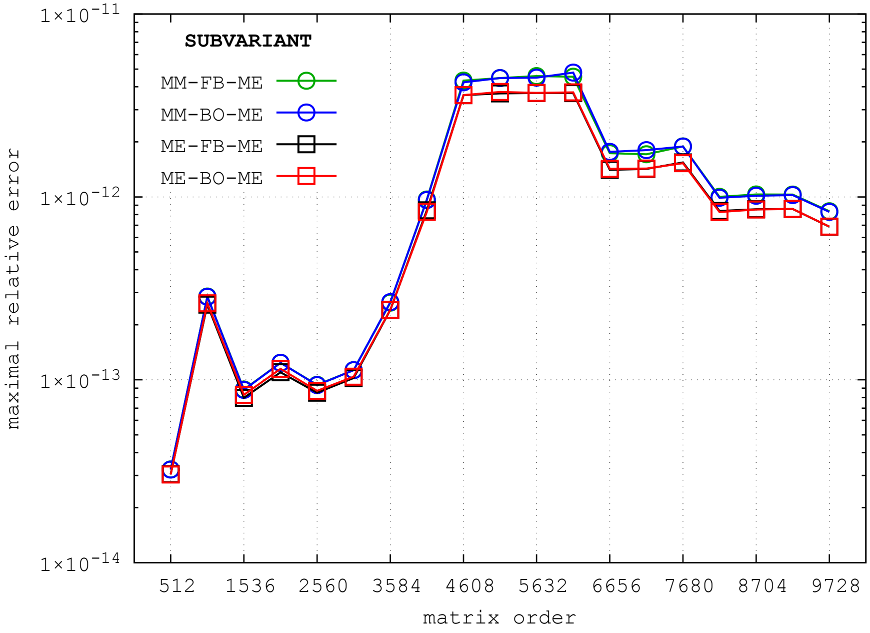


**Figure 41.** The maximal normwise relative error in the computed decomposition of the second matrix in a matrix pair, $\|G - V\Sigma_G X\|_F / \|G\|_F$, for the Algorithm **DHZ6** on the matrices from the test set, with orders varying from $512$ to $9728$.

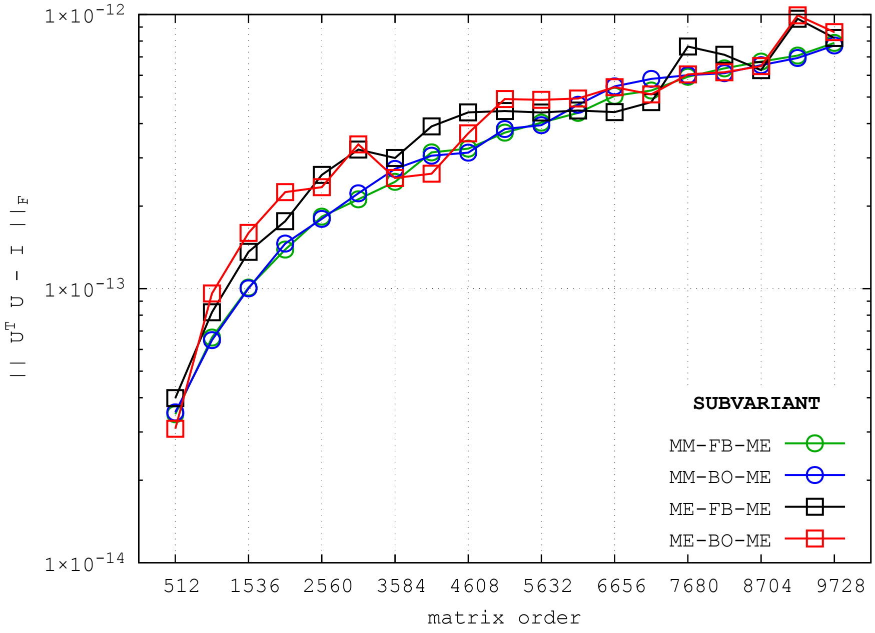


**Figure 42.** Orthogonality $\|U^T U - I\|_F$ of the left generalized singular vectors $U$ for the Algorithm **DHZ6** on the matrices from the test set, with orders varying from $512$ to $9728$.

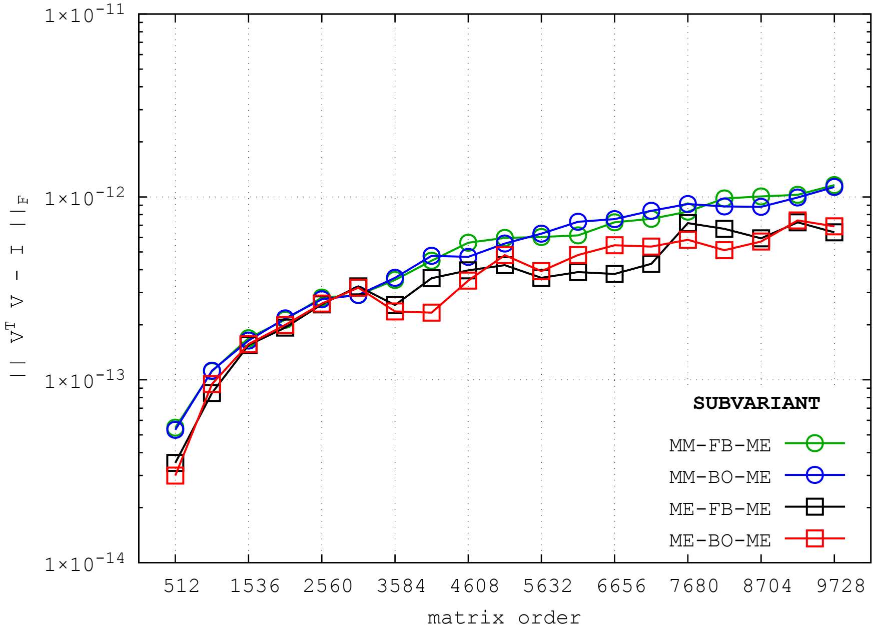


**Figure 43.** Orthogonality $\|V^T V - I\|_F$ of the left generalized singular vectors $V$ for the Algorithm **DHZ6** on the matrices from the test set, with orders varying from $512$ to $9728$.

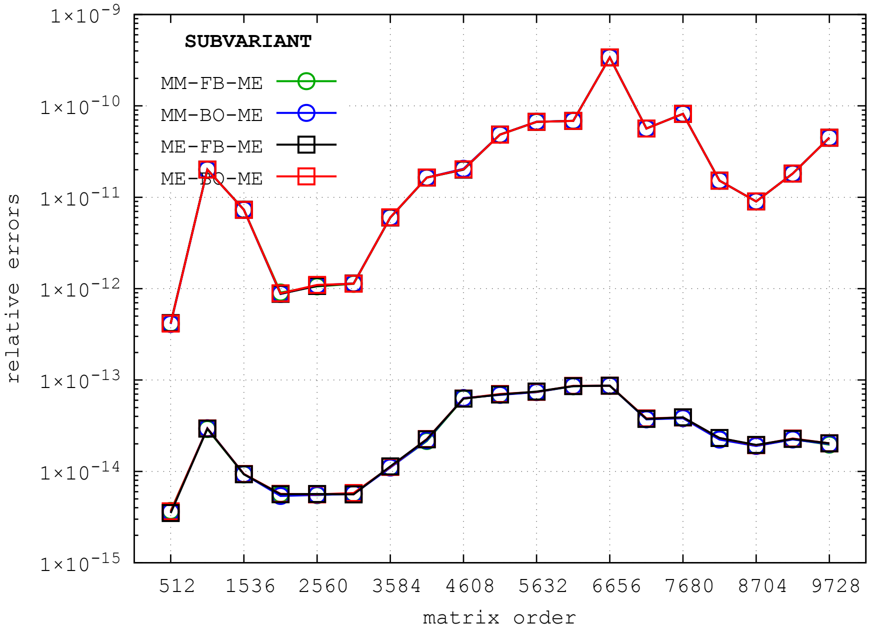


**Figure 44.** The maximal (upper graph) and the average (lower graph) relative errors in the computed versus the original generalized singular values for the Algorithm **DHZ6** on the matrices from the test set, with orders varying from $512$ to $9728$. Neither the choice of a DHZ variant, nor of an outer Jacobi strategy, affects the errors much in those test cases.

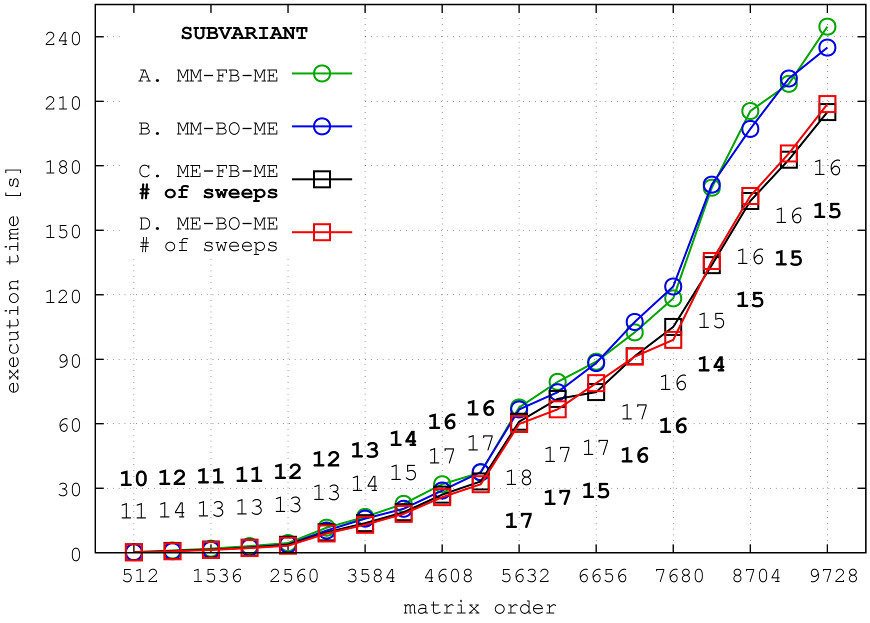


**Figure 45.** The wall execution time and the number of block sweeps for the the block-oriented (BO) and the full block (FB) DHZ variants, with the outer Jacobi strategies chosen as ME or MM (the inner strategy always being ME), for the Algorithm **DHZ7** and the matrices from the test set, with orders varying from $512$ to $9728$. The number of sweeps is shown for the ME-BO and the ME-FB (in **bold**). For the MM strategy those numbers are usually larger than for the corresponding ME-using variant.

### 2.1.8 *DHZ7*

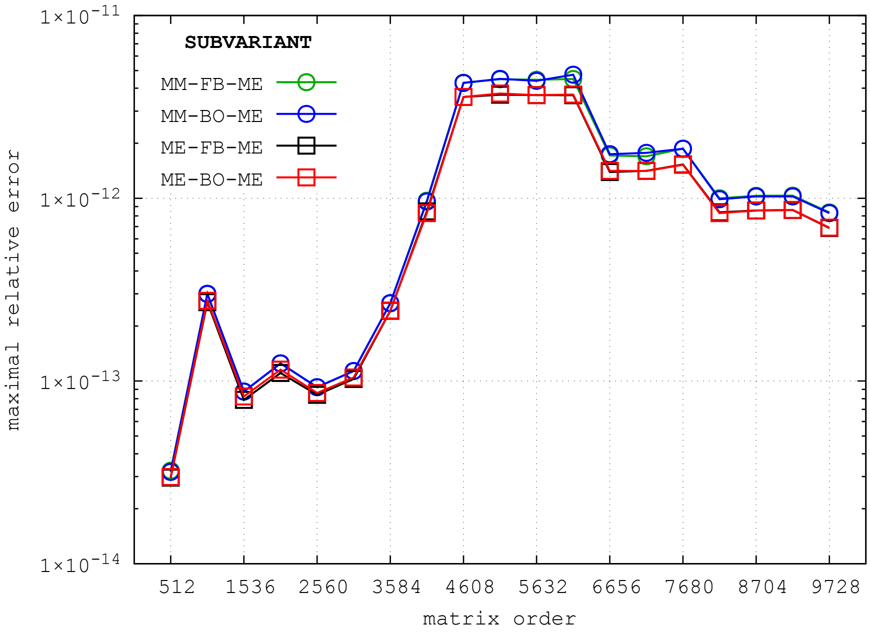


**Figure 46.** The maximal normwise relative error in the computed decomposition of the first matrix in a matrix pair, $\|F - U\Sigma_F X\|_F / \|F\|_F$, for the Algorithm **DHZ7** on the matrices from the test set, with orders varying from $512$ to $9728$.

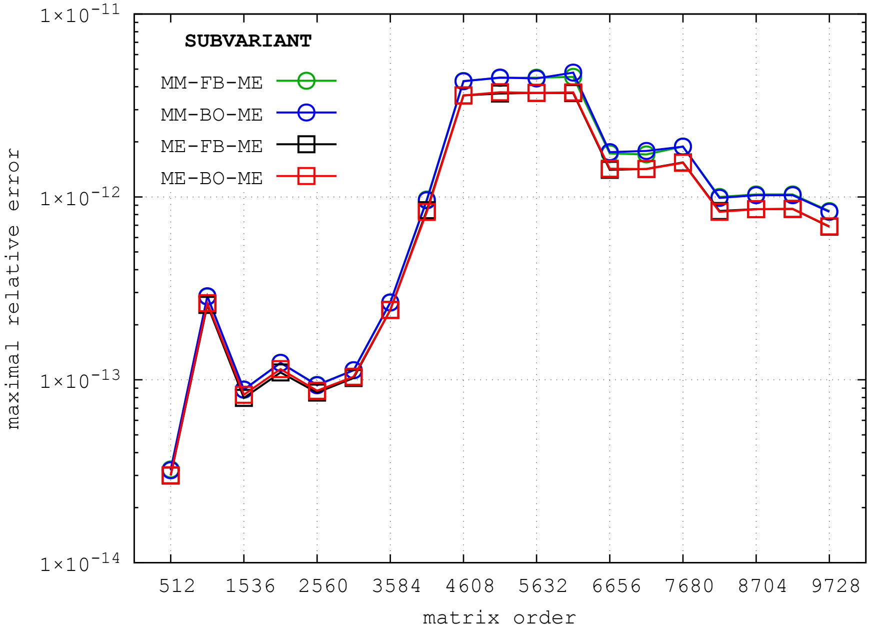


**Figure 47.** The maximal normwise relative error in the computed decomposition of the second matrix in a matrix pair, $\|G - V\Sigma_G X\|_F / \|G\|_F$, for the Algorithm **DHZ7** on the matrices from the test set, with orders varying from $512$ to $9728$.

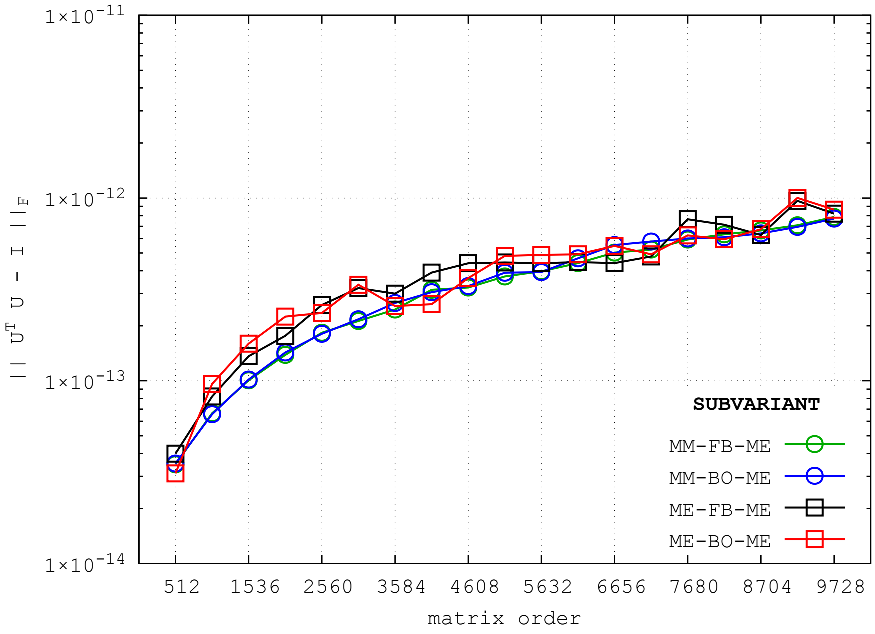


**Figure 48.** Orthogonality $\|U^T U - I\|_F$ of the left generalized singular vectors $U$ for the Algorithm **DHZ7** on the matrices from the test set, with orders varying from $512$ to $9728$.

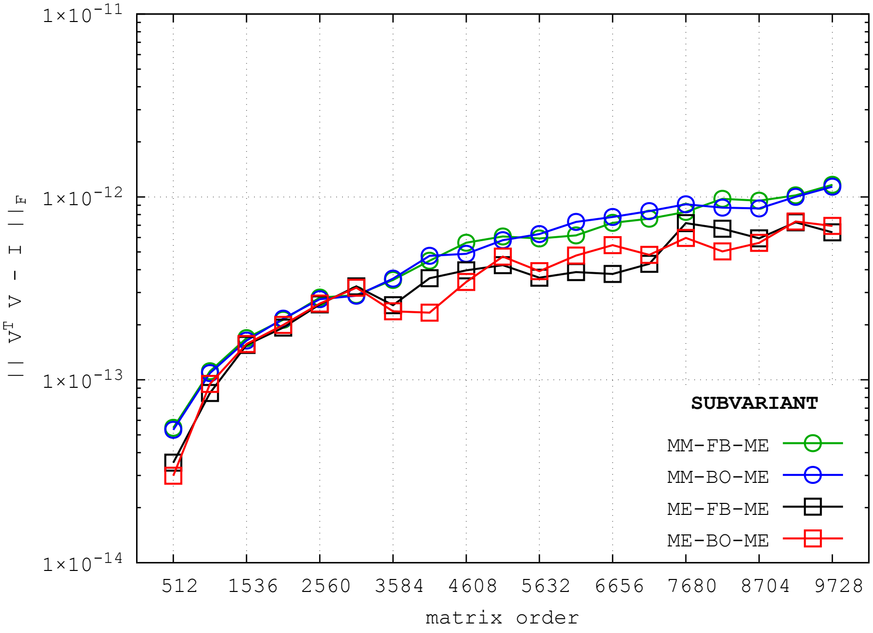


**Figure 49.** Orthogonality $\|V^TV - I\|_F$ of the left generalized singular vectors $V$ for the Algorithm **DHZ7** on the matrices from the test set, with orders varying from $512$ to $9728$.

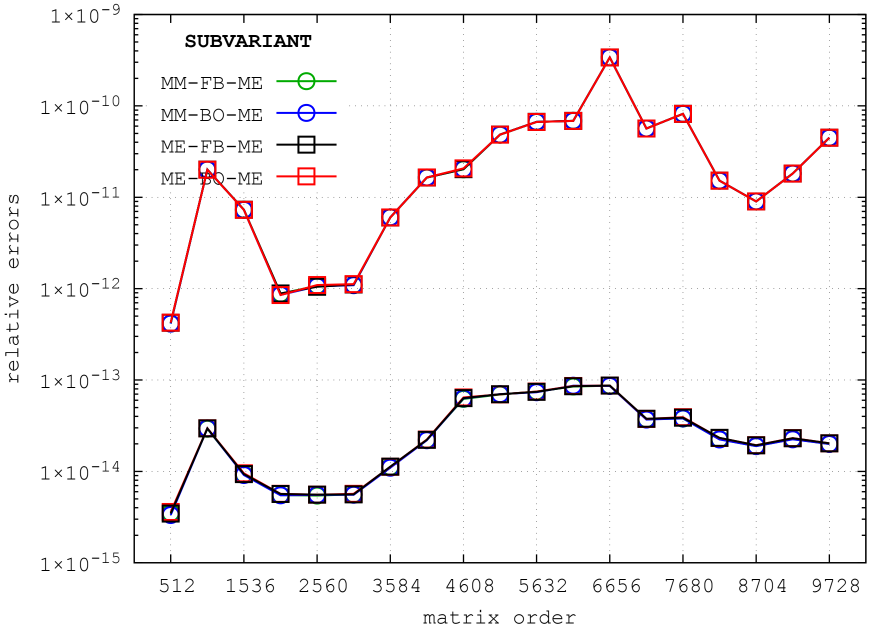


**Figure 50.** The maximal (upper graph) and the average (lower graph) relative errors in the computed versus the original generalized singular values for the Algorithm **DHZ7** on the matrices from the test set, with orders varying from $512$ to $9728$. Neither the choice of a DHZ variant, nor of an outer Jacobi strategy, affects the errors much in those test cases.

## *2.2 ZHZ*

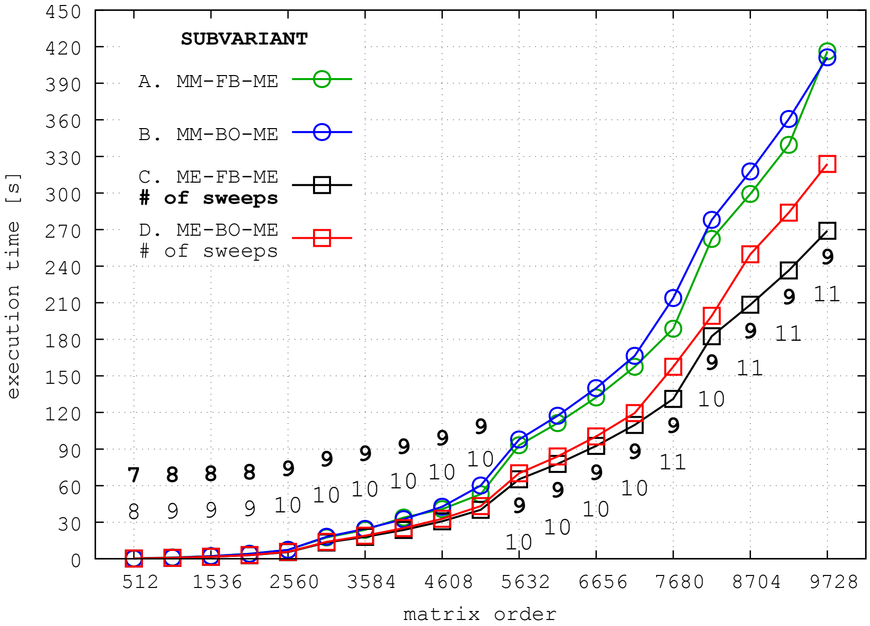


**Figure 51.** The wall execution time and the number of block sweeps for the the block-oriented (BO) and the full block (FB) ZHZ variants, with the outer Jacobi strategies chosen as ME or MM (the inner strategy always being ME), for the Algorithm **ZHZ0** and the matrices from the test set, with orders varying from $512$ to $9728$. The number of sweeps is shown for the ME-BO and the ME-FB (in **bold**). For the MM strategy those numbers are usually larger than for the corresponding ME-using variant.

### *2.2.1 ZHZ0*

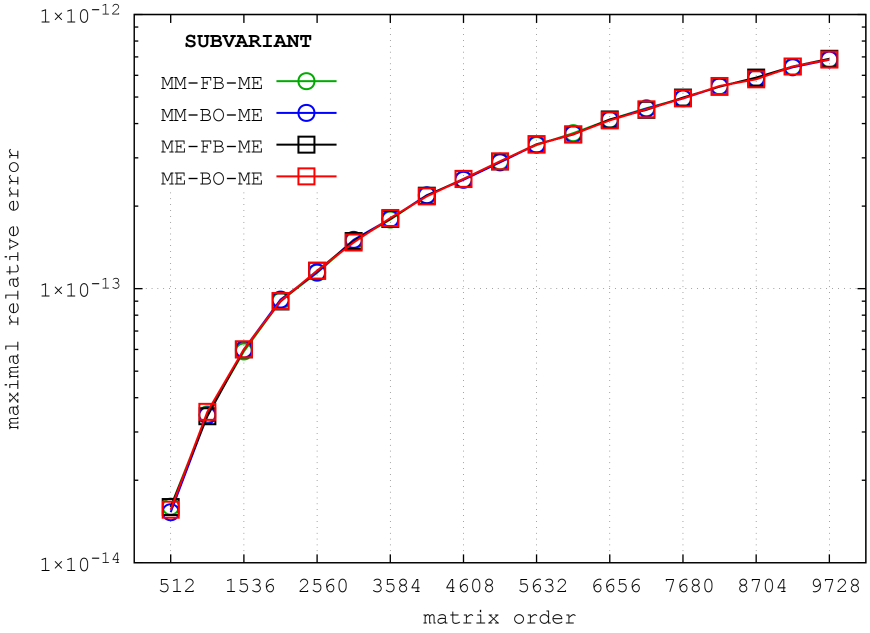


**Figure 52.** The maximal normwise relative error in the computed decomposition of the first matrix in a matrix pair, $\|F - U\Sigma_F X\|_F / \|F\|_F$, for the Algorithm **ZHZ0** on the matrices from the test set, with orders varying from $512$ to $9728$.

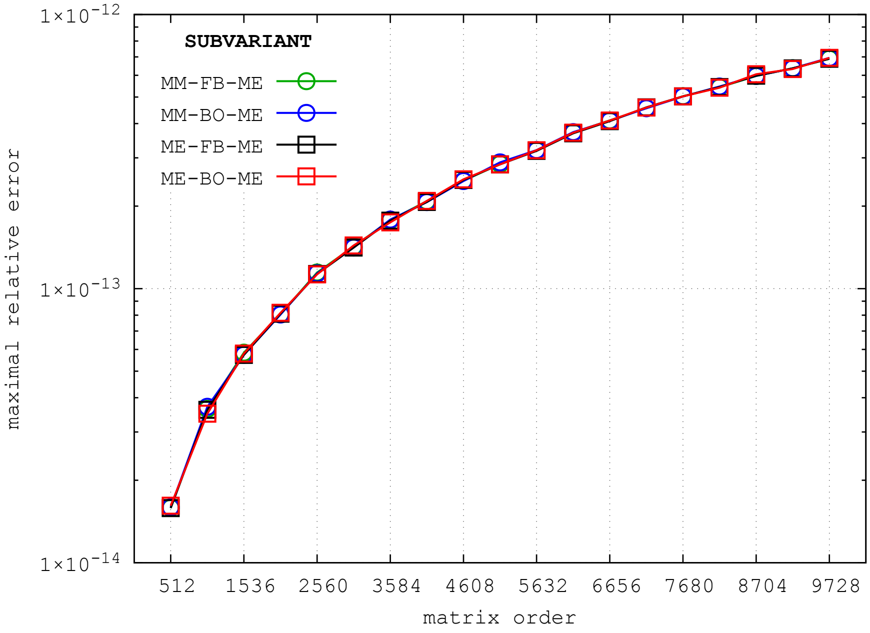


**Figure 53.** The maximal normwise relative error in the computed decomposition of the second matrix in a matrix pair, $\|G - V\Sigma_G X\|_F / \|G\|_F$, for the Algorithm **ZHZ0** on the matrices from the test set, with orders varying from $512$ to $9728$.

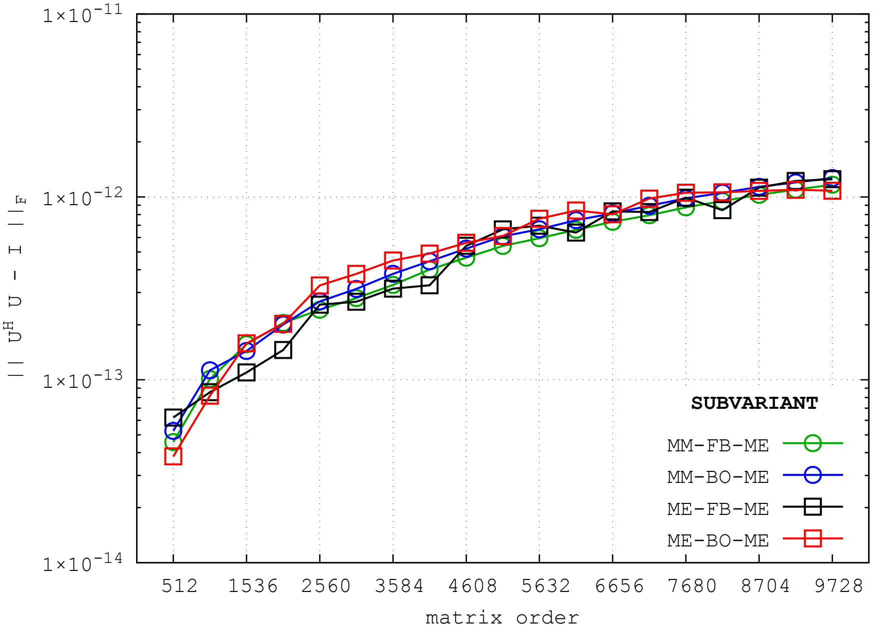


**Figure 54.** Orthogonality $\|U^{*}U - I\|_F$ of the left generalized singular vectors $U$ for the Algorithm **ZHZ0** on the matrices from the test set, with orders varying from $512$ to $9728$.

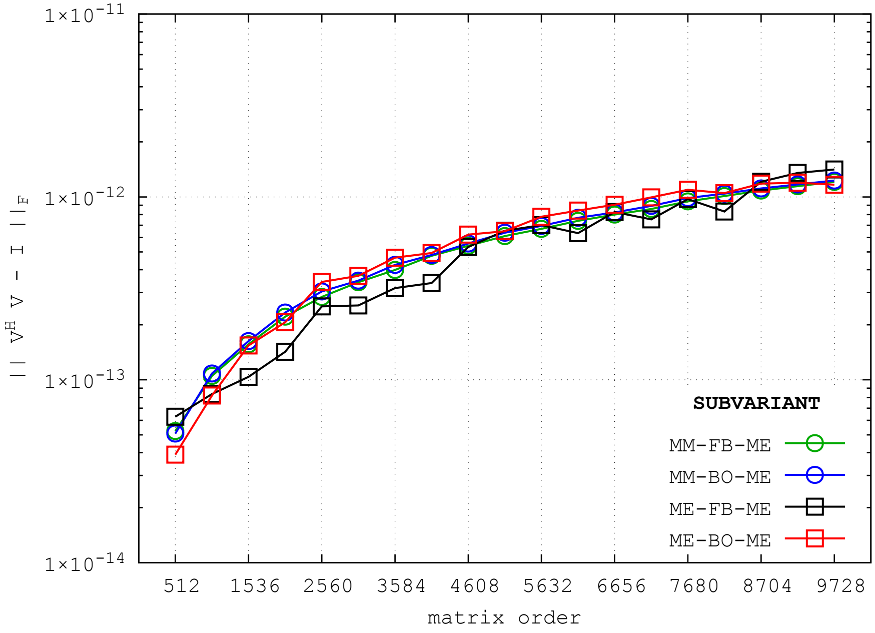


**Figure 55.** Orthogonality $\|V^*V - I\|_F$ of the left generalized singular vectors $V$ for the Algorithm **ZHZ0** on the matrices from the test set, with orders varying from $512$ to $9728$.

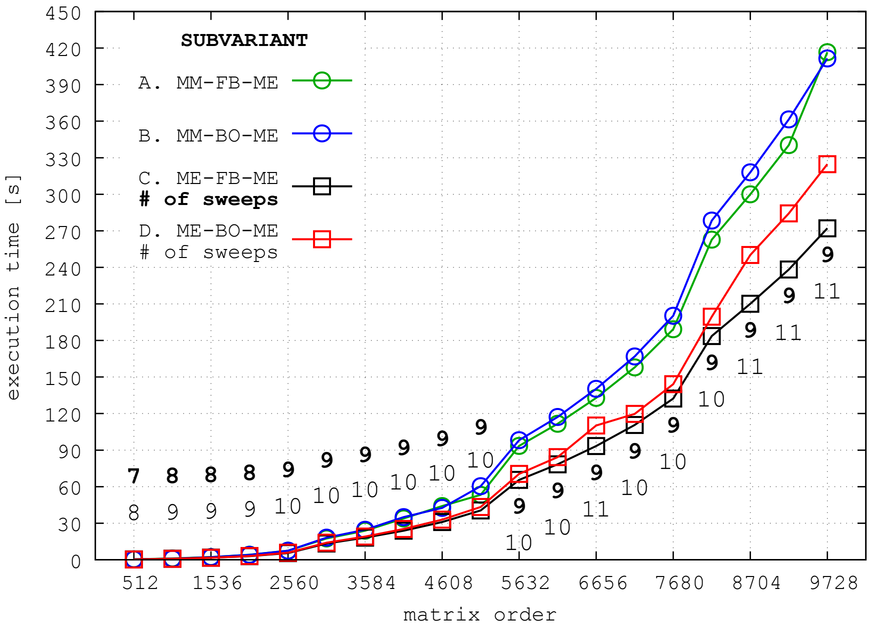


**Figure 56.** The wall execution time and the number of block sweeps for the the block-oriented (BO) and the full block (FB) ZHZ variants, with the outer Jacobi strategies chosen as ME or MM (the inner strategy always being ME), for the Algorithm **ZHZ1** and the matrices from the test set, with orders varying from $512$ to $9728$. The number of sweeps is shown for the ME-BO and the ME-FB (in **bold**). For the MM strategy those numbers are usually larger than for the corresponding ME-using variant.

### *2.2.2 ZHZ1*

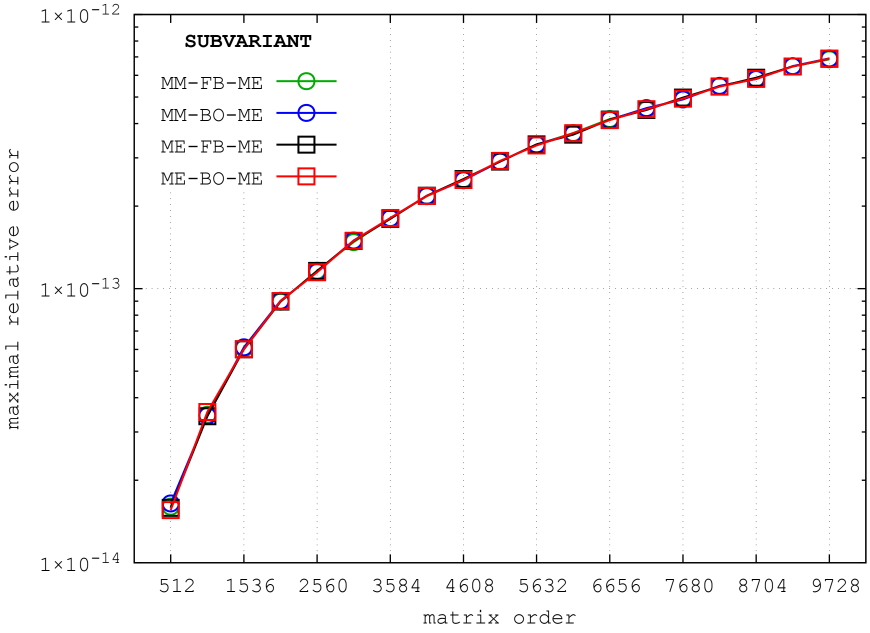


**Figure 57.** The maximal normwise relative error in the computed decomposition of the first matrix in a matrix pair, $\|F - U\Sigma_F X\|_F / \|F\|_F$, for the Algorithm **ZHZ1** on the matrices from the test set, with orders varying from $512$ to $9728$.

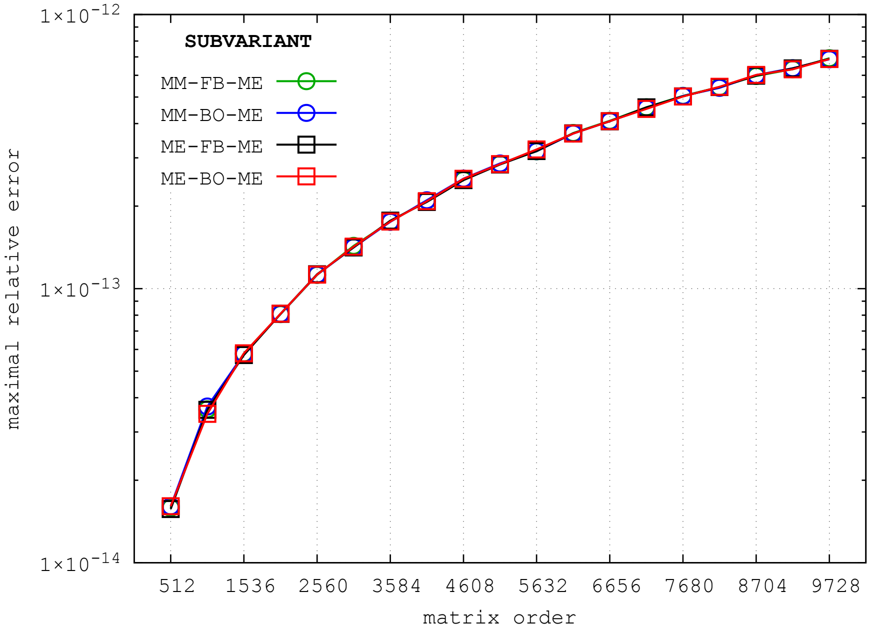


**Figure 58.** The maximal normwise relative error in the computed decomposition of the second matrix in a matrix pair, $\|G - V\Sigma_G X\|_F / \|G\|_F$, for the Algorithm **ZHZ1** on the matrices from the test set, with orders varying from $512$ to $9728$.

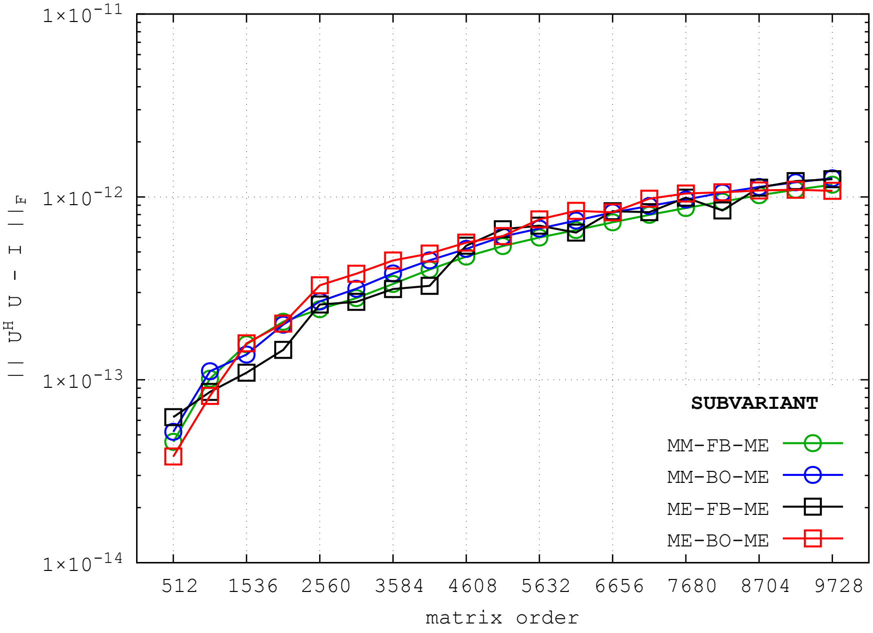


**Figure 59.** Orthogonality $\|U^*U - I\|_F$ of the left generalized singular vectors $U$ for the Algorithm **ZHZ1** on the matrices from the test set, with orders varying from $512$ to $9728$.

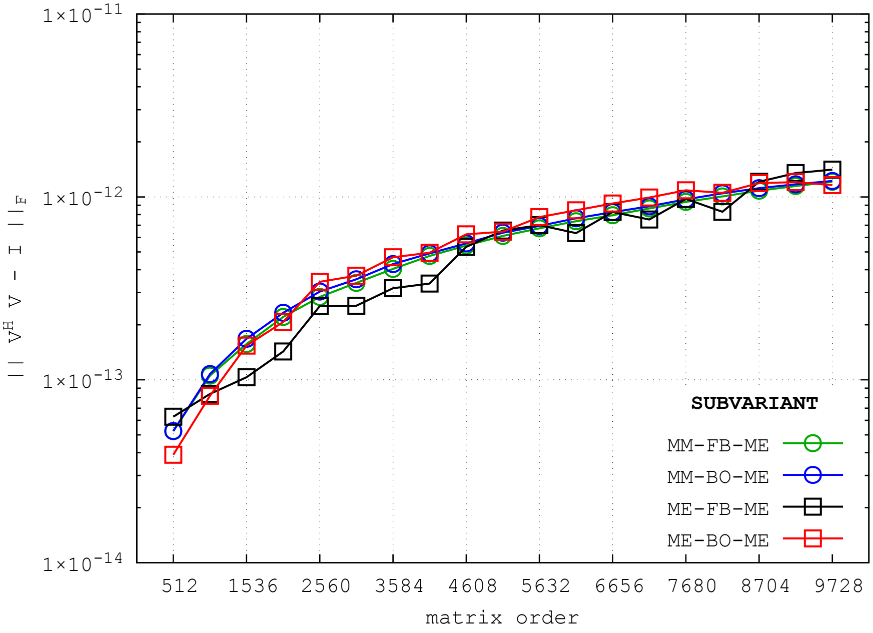


**Figure 60.** Orthogonality $\|V^*V - I\|_F$ of the left generalized singular vectors $V$ for the Algorithm **ZHZ1** on the matrices from the test set, with orders varying from $512$ to $9728$.

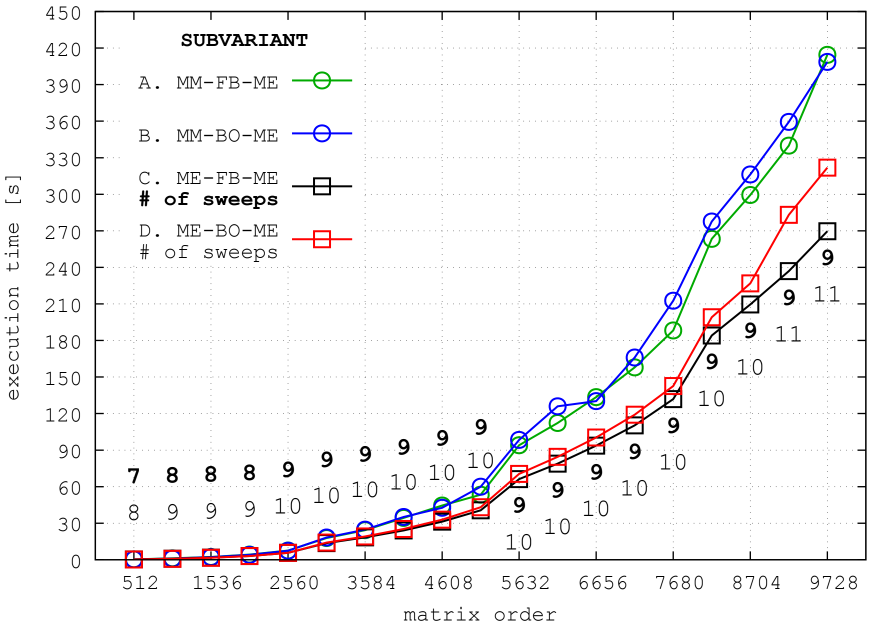


**Figure 61.** The wall execution time and the number of block sweeps for the the block-oriented (BO) and the full block (FB) ZHZ variants, with the outer Jacobi strategies chosen as ME or MM (the inner strategy always being ME), for the Algorithm **ZHZ2** and the matrices from the test set, with orders varying from $512$ to $9728$. The number of sweeps is shown for the ME-BO and the ME-FB (in **bold**). For the MM strategy those numbers are usually larger than for the corresponding ME-using variant.

### 2.2.3 *ZHZ2*

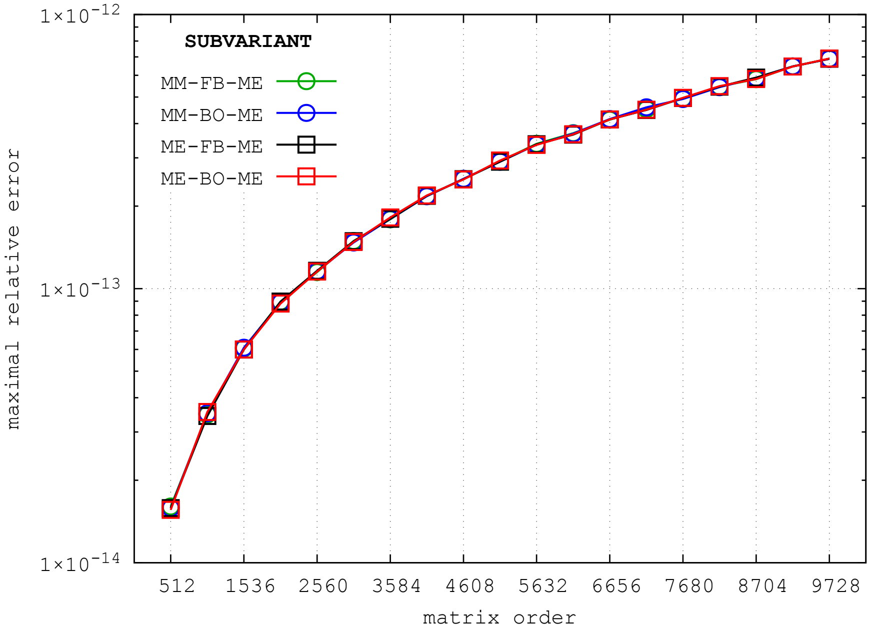


**Figure 62.** The maximal normwise relative error in the computed decomposition of the first matrix in a matrix pair, $\|F - U\Sigma_F X\|_F / \|F\|_F$, for the Algorithm **ZHZ2** on the matrices from the test set, with orders varying from $512$ to $9728$.

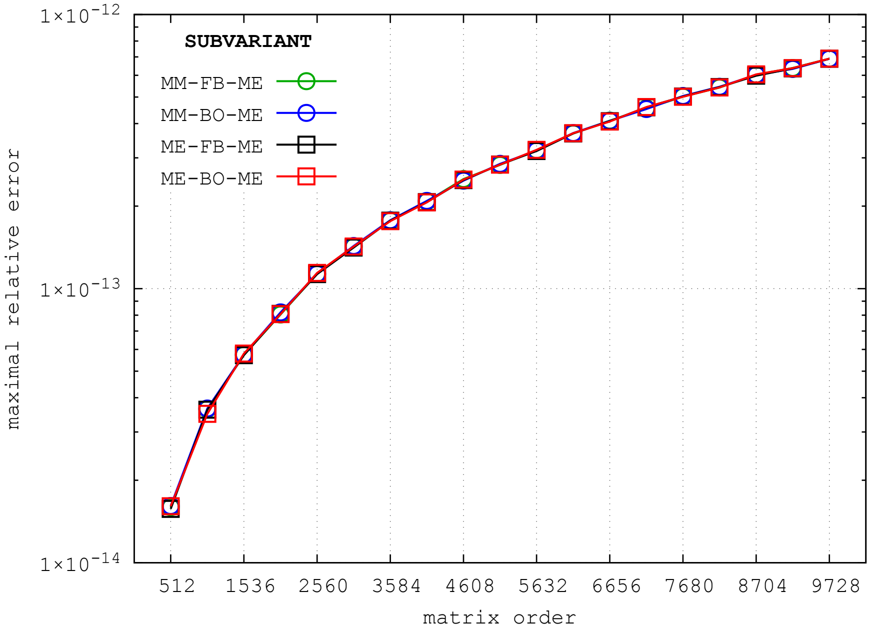


**Figure 63.** The maximal normwise relative error in the computed decomposition of the second matrix in a matrix pair, $\|G - V\Sigma_G X\|_F / \|G\|_F$, for the Algorithm **ZHZ2** on the matrices from the test set, with orders varying from $512$ to $9728$.

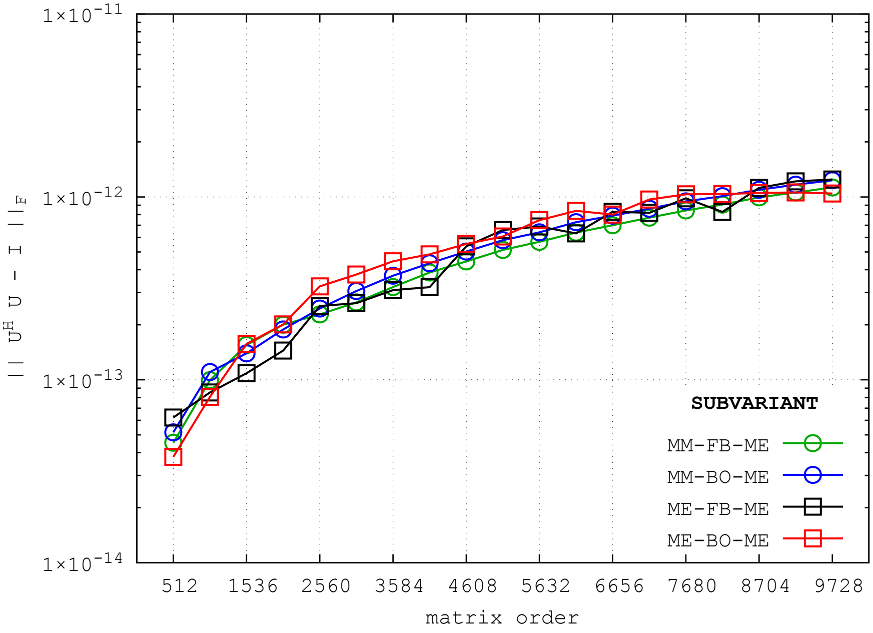


**Figure 64.** Orthogonality $\|U^*U - I\|_F$ of the left generalized singular vectors $U$ for the Algorithm **ZHZ2** on the matrices from the test set, with orders varying from $512$ to $9728$.

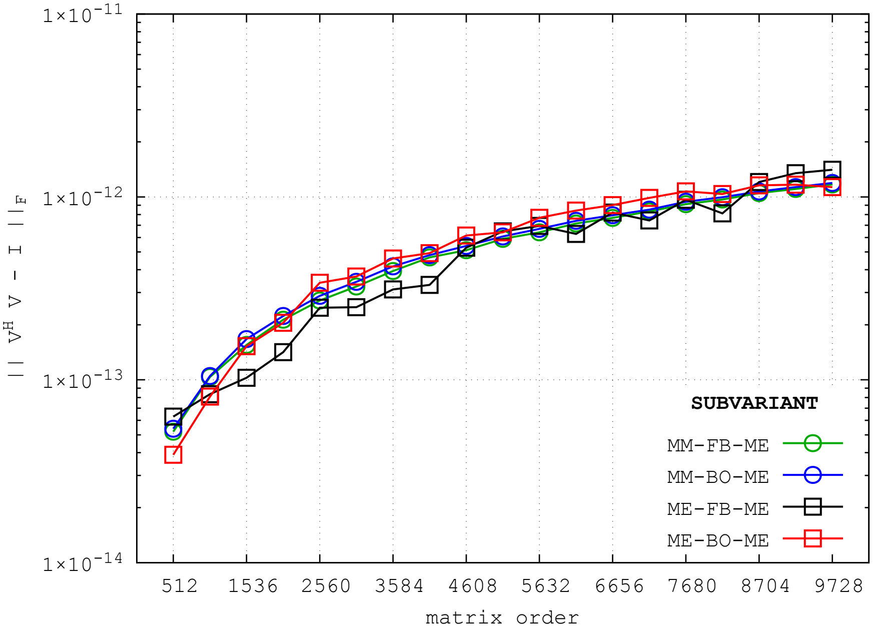


**Figure 65.** Orthogonality $\|V^*V - I\|_F$ of the left generalized singular vectors $V$ for the Algorithm **ZHZ2** on the matrices from the test set, with orders varying from $512$ to $9728$.

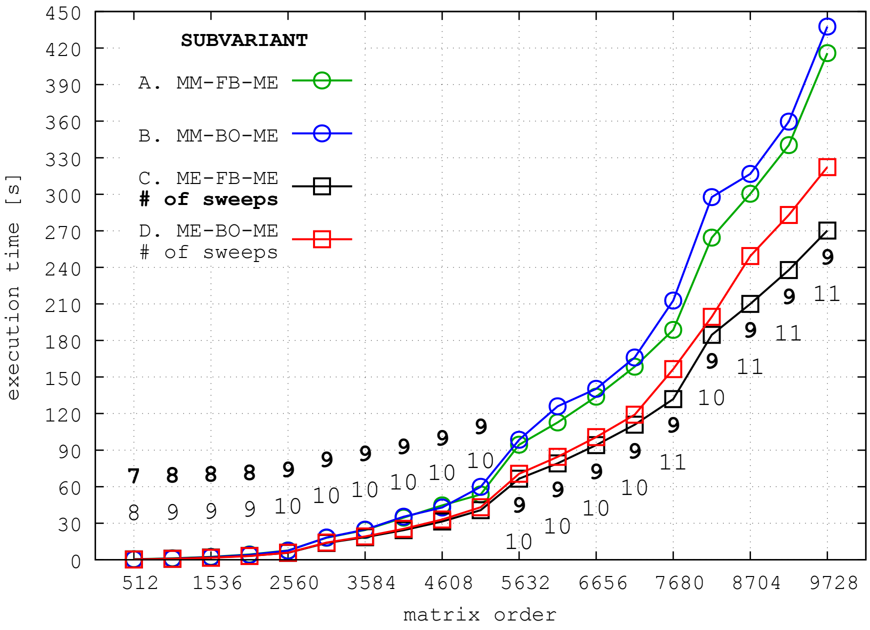


**Figure 66.** The wall execution time and the number of block sweeps for the the block-oriented (BO) and the full block (FB) ZHZ variants, with the outer Jacobi strategies chosen as ME or MM (the inner strategy always being ME), for the Algorithm **ZHZ3** and the matrices from the test set, with orders varying from $512$ to $9728$. The number of sweeps is shown for the ME-BO and the ME-FB (in **bold**). For the MM strategy those numbers are usually larger than for the corresponding ME-using variant.

### *2.2.4 ZHZ3*

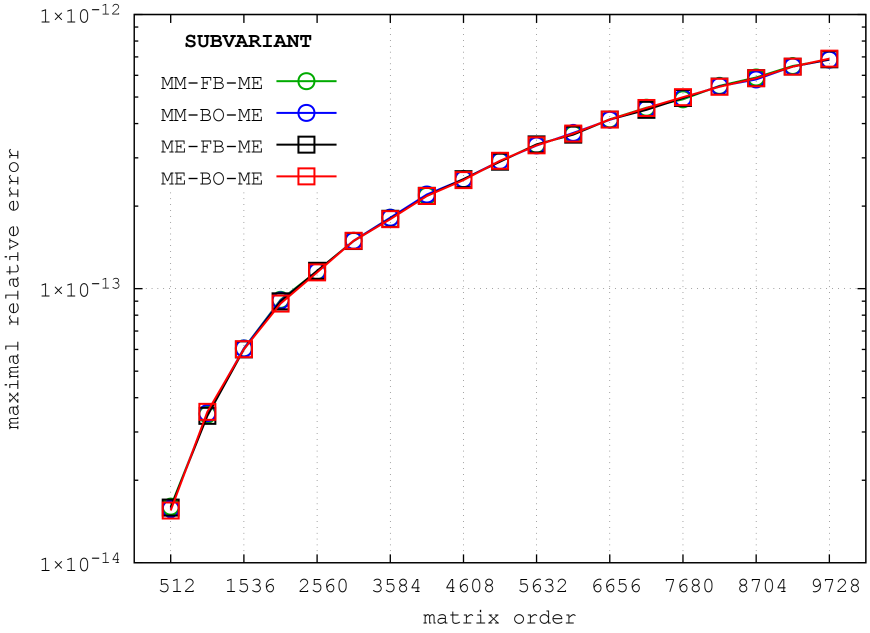


**Figure 67.** The maximal normwise relative error in the computed decomposition of the first matrix in a matrix pair, $\|F - U\Sigma_F X\|_F / \|F\|_F$, for the Algorithm **ZHZ3** on the matrices from the test set, with orders varying from $512$ to $9728$.

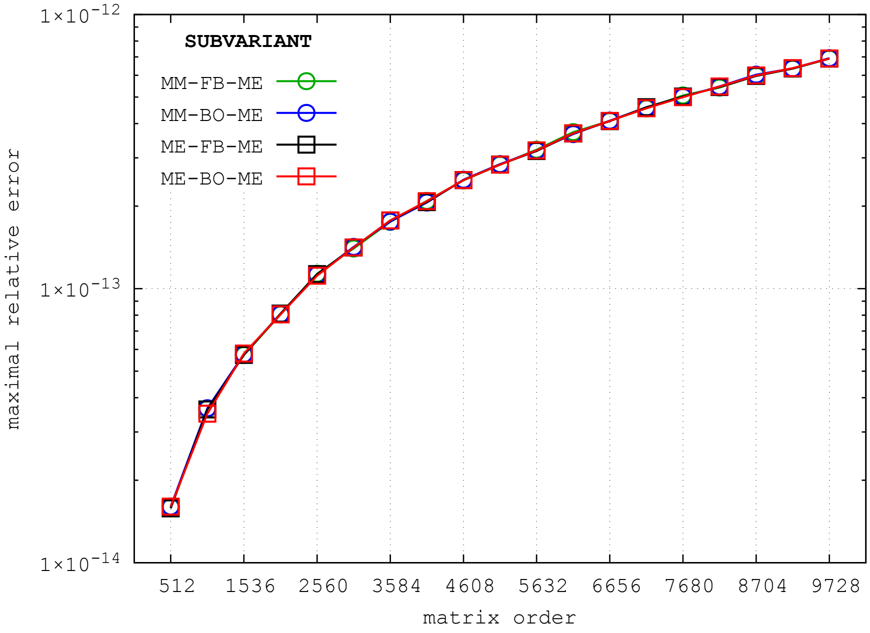


**Figure 68.** The maximal normwise relative error in the computed decomposition of the second matrix in a matrix pair, $\|G - V\Sigma_G X\|_F / \|G\|_F$, for the Algorithm **ZHZ3** on the matrices from the test set, with orders varying from $512$ to $9728$.

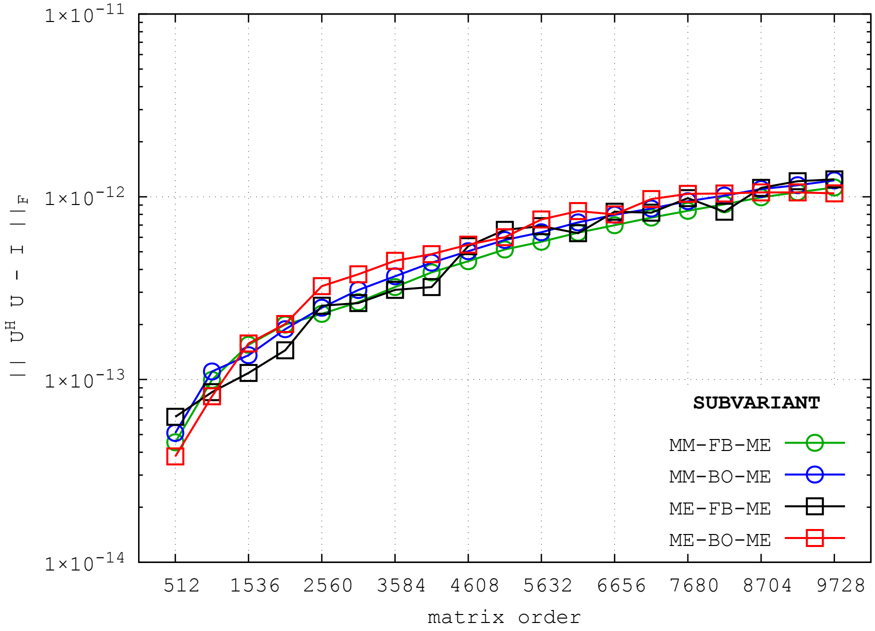


**Figure 69.** Orthogonality $\|U^*U - I\|_F$ of the left generalized singular vectors $U$ for the Algorithm **ZHZ3** on the matrices from the test set, with orders varying from $512$ to $9728$.

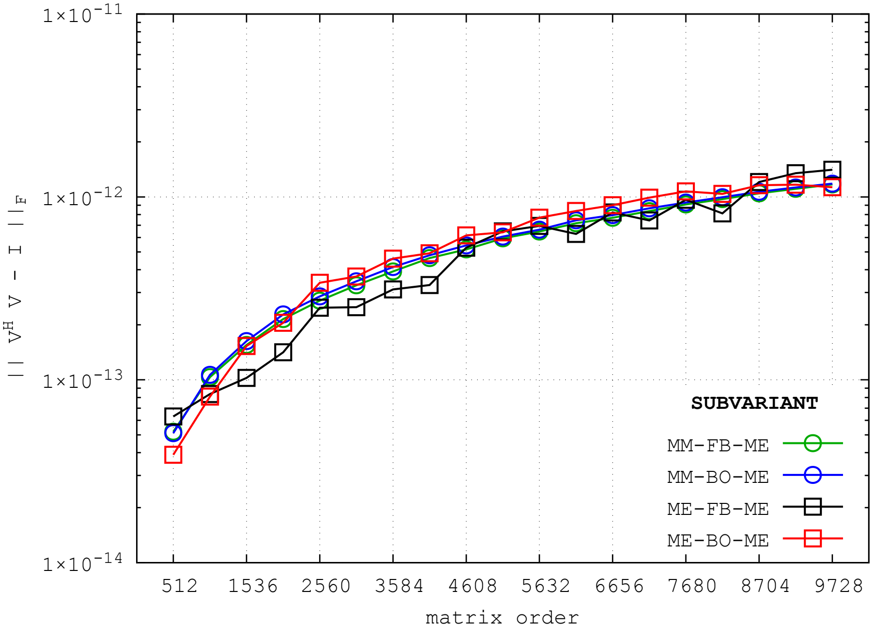


**Figure 70.** Orthogonality $\|V^*V - I\|_F$ of the left generalized singular vectors $V$ for the Algorithm **ZHZ3** on the matrices from the test set, with orders varying from $512$ to $9728$.

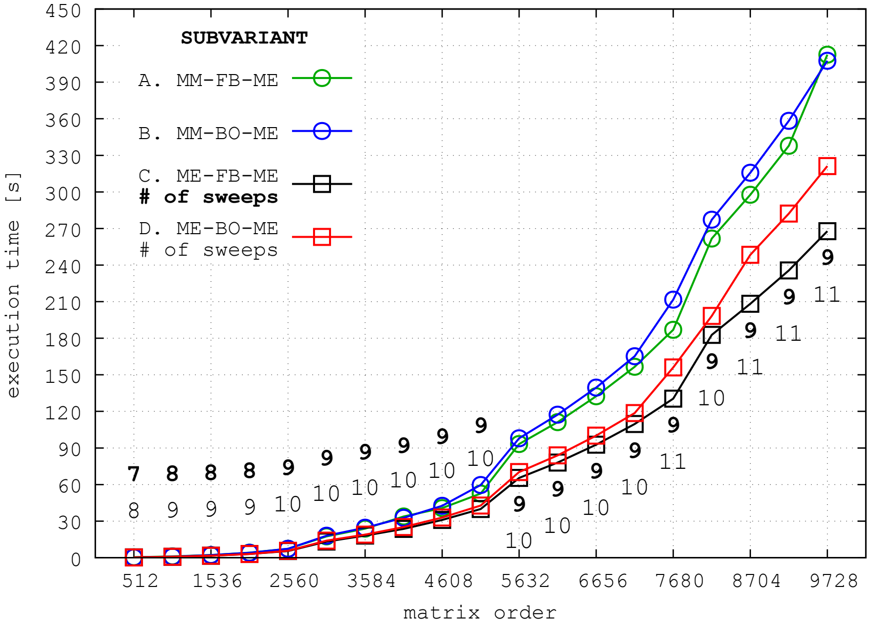


**Figure 71.** The wall execution time and the number of block sweeps for the the block-oriented (BO) and the full block (FB) ZHZ variants, with the outer Jacobi strategies chosen as ME or MM (the inner strategy always being ME), for the Algorithm **ZHZ4** and the matrices from the test set, with orders varying from $512$ to $9728$. The number of sweeps is shown for the ME-BO and the ME-FB (in **bold**). For the MM strategy those numbers are usually larger than for the corresponding ME-using variant.

### *2.2.5 ZHZ4*

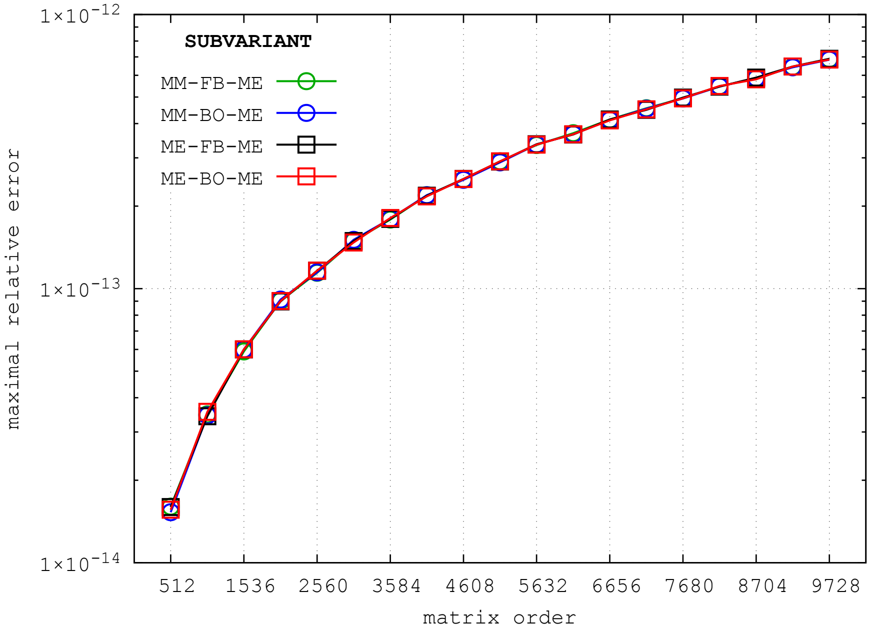


**Figure 72.** The maximal normwise relative error in the computed decomposition of the first matrix in a matrix pair, $\|F - U\Sigma_F X\|_F / \|F\|_F$, for the Algorithm **ZHZ4** on the matrices from the test set, with orders varying from $512$ to $9728$.

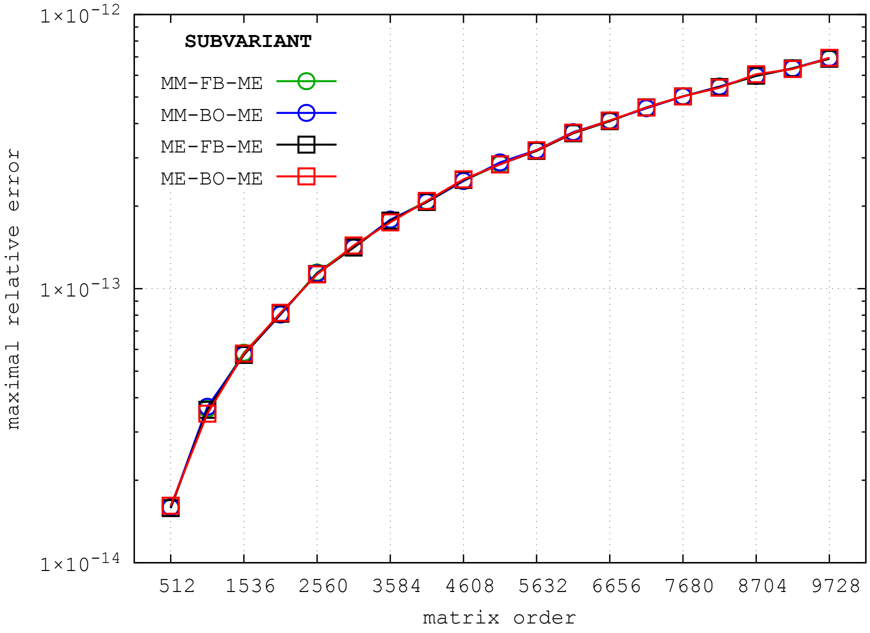


**Figure 73.** The maximal normwise relative error in the computed decomposition of the second matrix in a matrix pair, $\|G - V\Sigma_G X\|_F / \|G\|_F$, for the Algorithm **ZHZ4** on the matrices from the test set, with orders varying from $512$ to $9728$.

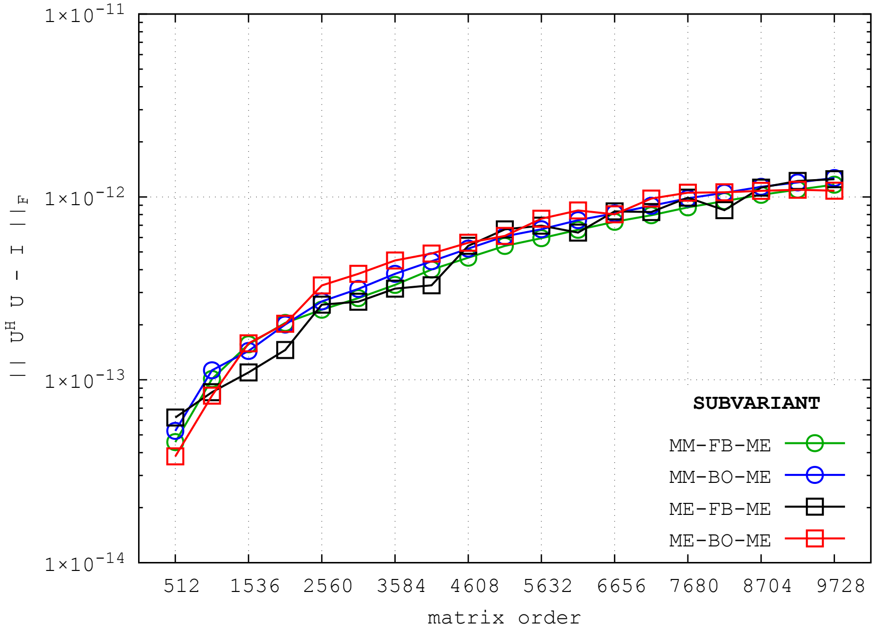


**Figure 74.** Orthogonality $\|U^*U - I\|_F$ of the left generalized singular vectors $U$ for the Algorithm **ZHZ4** on the matrices from the test set, with orders varying from $512$ to $9728$.

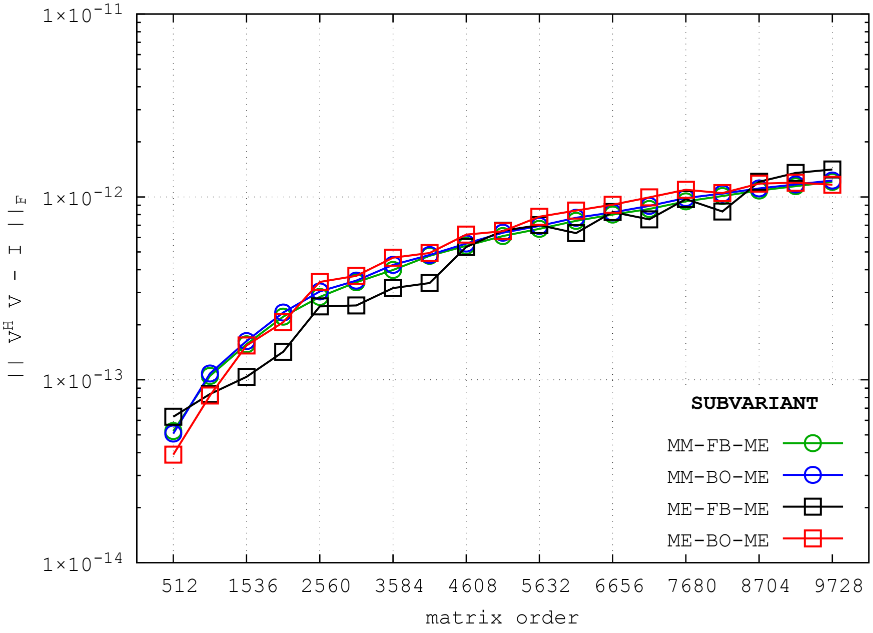


**Figure 75.** Orthogonality $\|V^*V - I\|_F$ of the left generalized singular vectors $V$ for the Algorithm **ZHZ4** on the matrices from the test set, with orders varying from $512$ to $9728$.

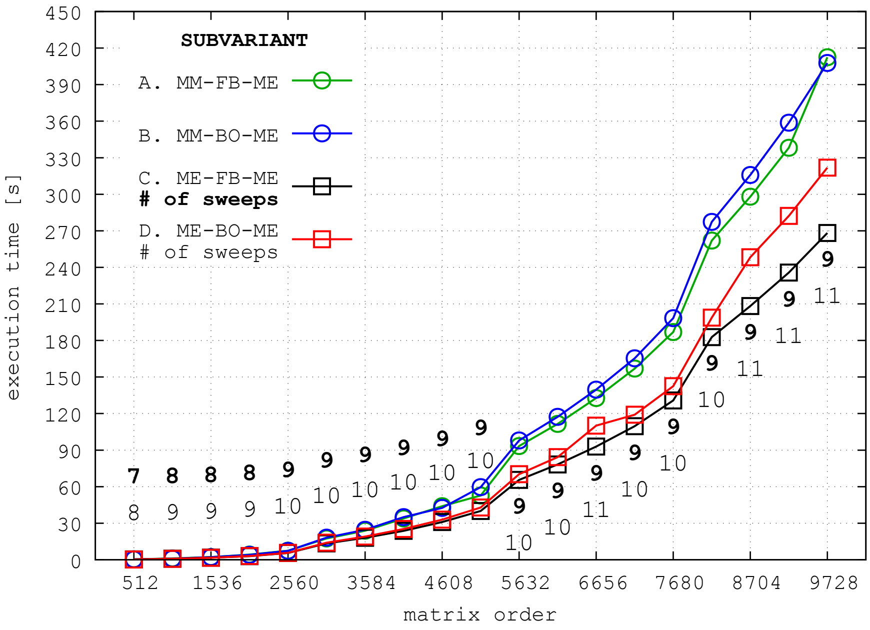


**Figure 76.** The wall execution time and the number of block sweeps for the the block-oriented (BO) and the full block (FB) ZHZ variants, with the outer Jacobi strategies chosen as ME or MM (the inner strategy always being ME), for the Algorithm **ZHZ5** and the matrices from the test set, with orders varying from $512$ to $9728$. The number of sweeps is shown for the ME-BO and the ME-FB (in **bold**). For the MM strategy those numbers are usually larger than for the corresponding ME-using variant.

### *2.2.6 ZHZ5*

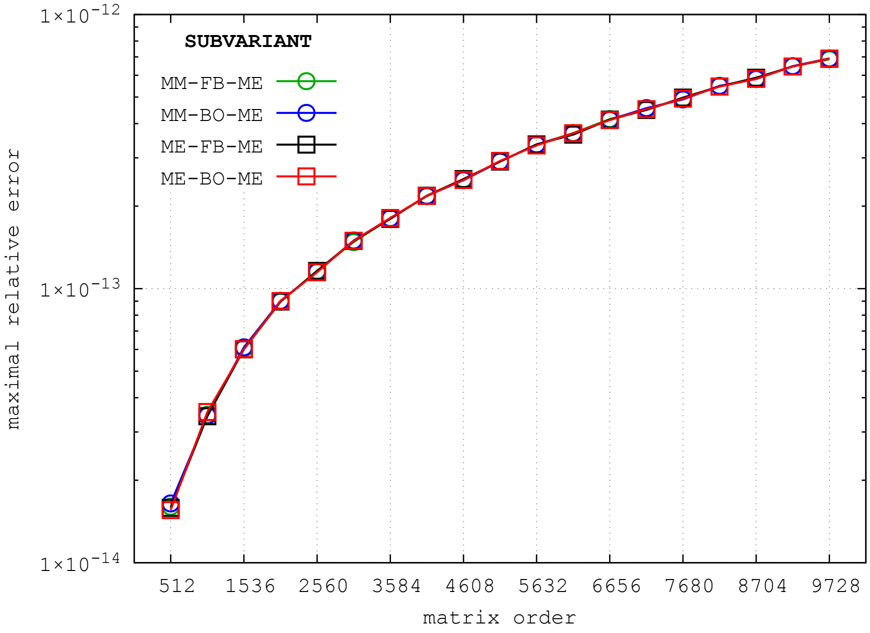


**Figure 77.** The maximal normwise relative error in the computed decomposition of the first matrix in a matrix pair, $\|F - U\Sigma_F X\|_F / \|F\|_F$, for the Algorithm **ZHZ5** on the matrices from the test set, with orders varying from $512$ to $9728$.

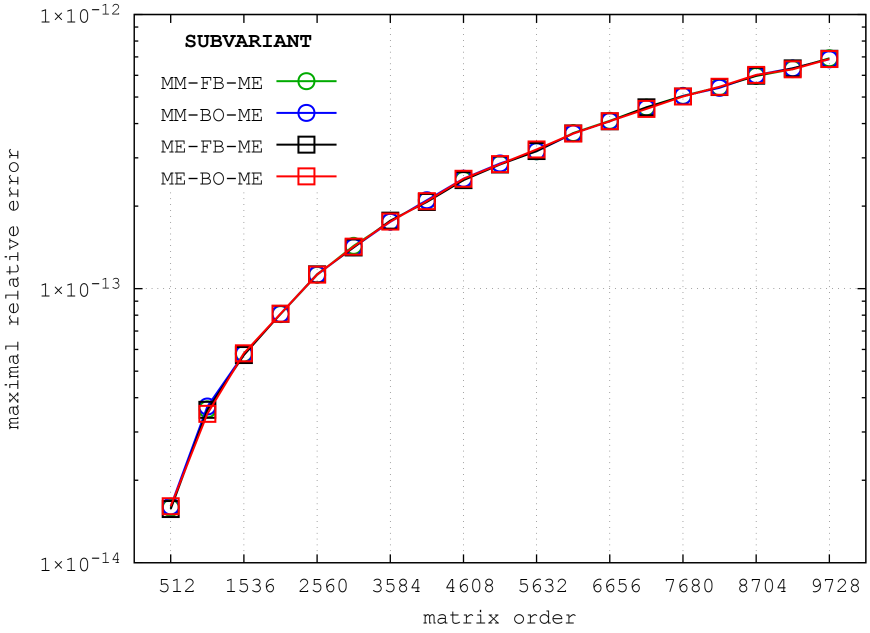


**Figure 78.** The maximal normwise relative error in the computed decomposition of the second matrix in a matrix pair, $\|G - V\Sigma_G X\|_F / \|G\|_F$, for the Algorithm **ZHZ5** on the matrices from the test set, with orders varying from $512$ to $9728$.

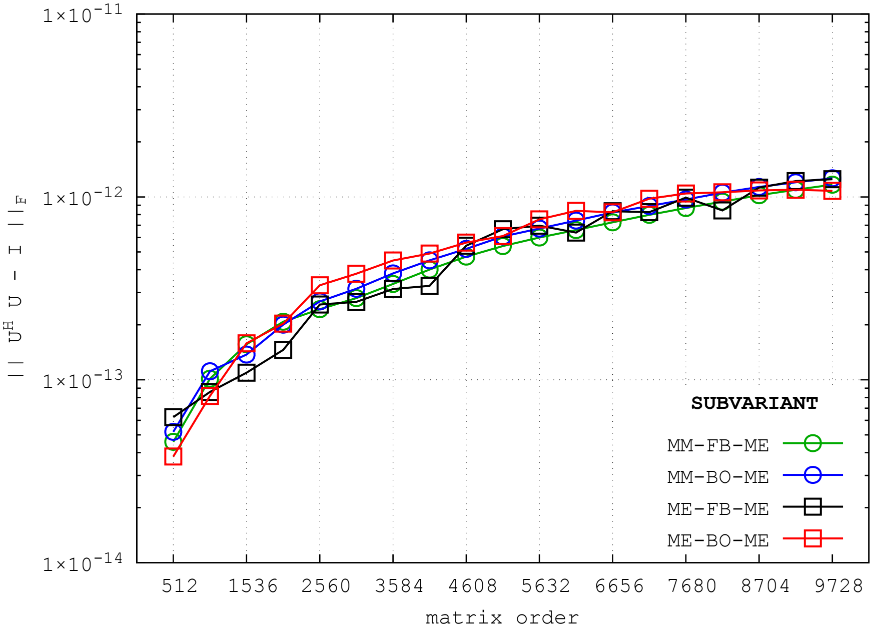


**Figure 79.** Orthogonality $\|U^*U - I\|_F$ of the left generalized singular vectors $U$ for the Algorithm **ZHZ5** on the matrices from the test set, with orders varying from $512$ to $9728$.

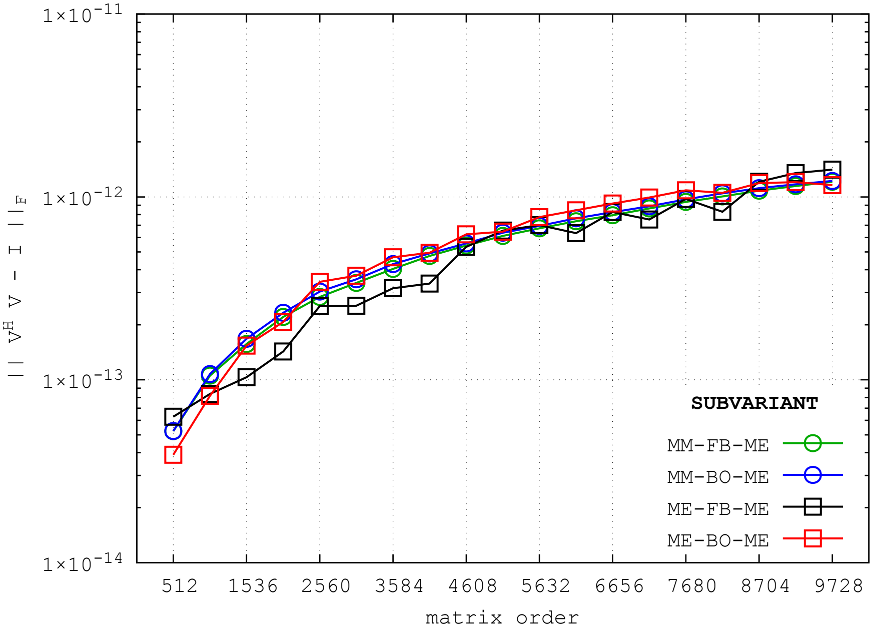


**Figure 80.** Orthogonality $\|V^*V - I\|_F$ of the left generalized singular vectors $V$ for the Algorithm **ZHZ5** on the matrices from the test set, with orders varying from $512$ to $9728$.

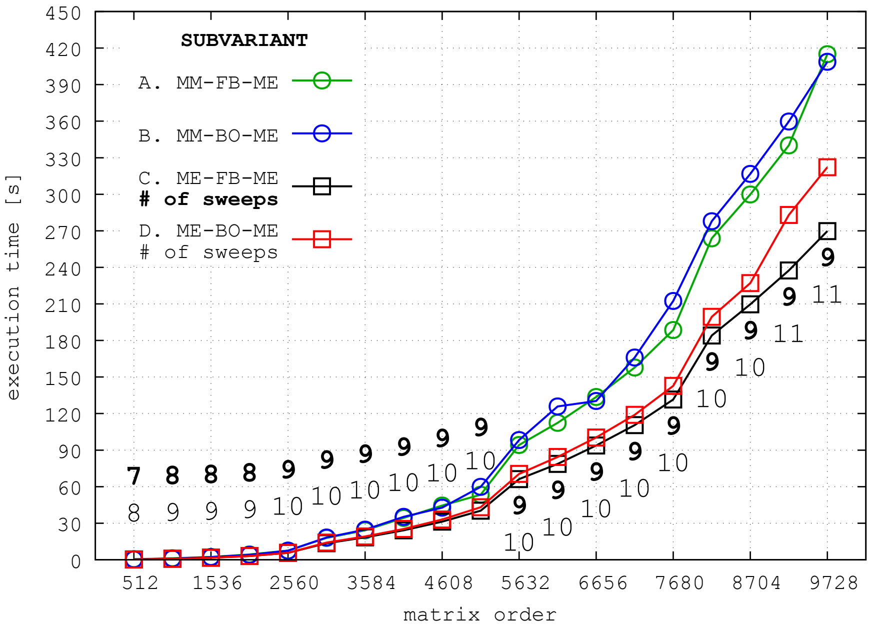


**Figure 81.** The wall execution time and the number of block sweeps for the the block-oriented (BO) and the full block (FB) ZHZ variants, with the outer Jacobi strategies chosen as ME or MM (the inner strategy always being ME), for the Algorithm **ZHZ6** and the matrices from the test set, with orders varying from $512$ to $9728$. The number of sweeps is shown for the ME-BO and the ME-FB (in **bold**). For the MM strategy those numbers are usually larger than for the corresponding ME-using variant.

### 2.2.7 *ZHZ6*

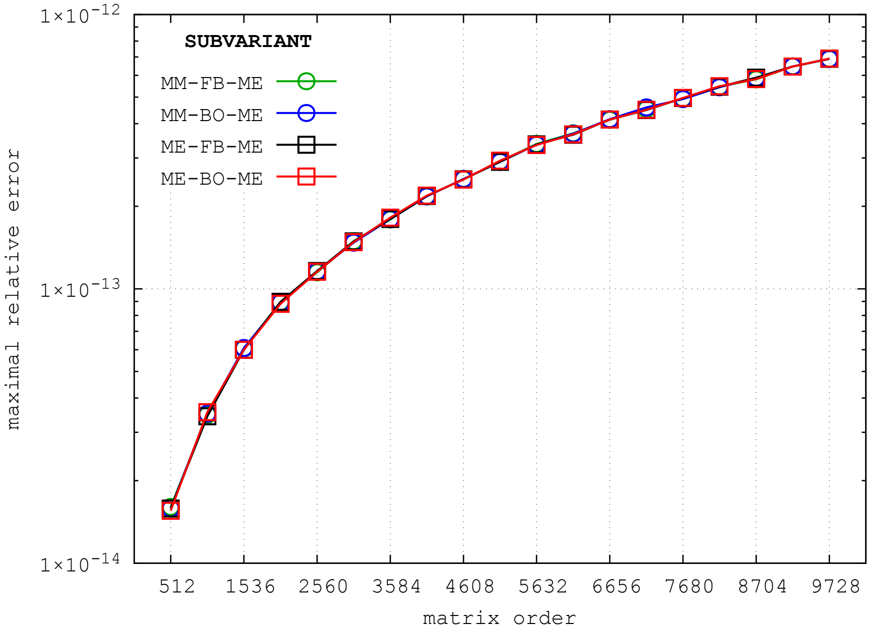


**Figure 82.** The maximal normwise relative error in the computed decomposition of the first matrix in a matrix pair, $\|F - U\Sigma_F X\|_F/\|F\|_F$, for the Algorithm **ZHZ6** on the matrices from the test set, with orders varying from $512$ to $9728$.

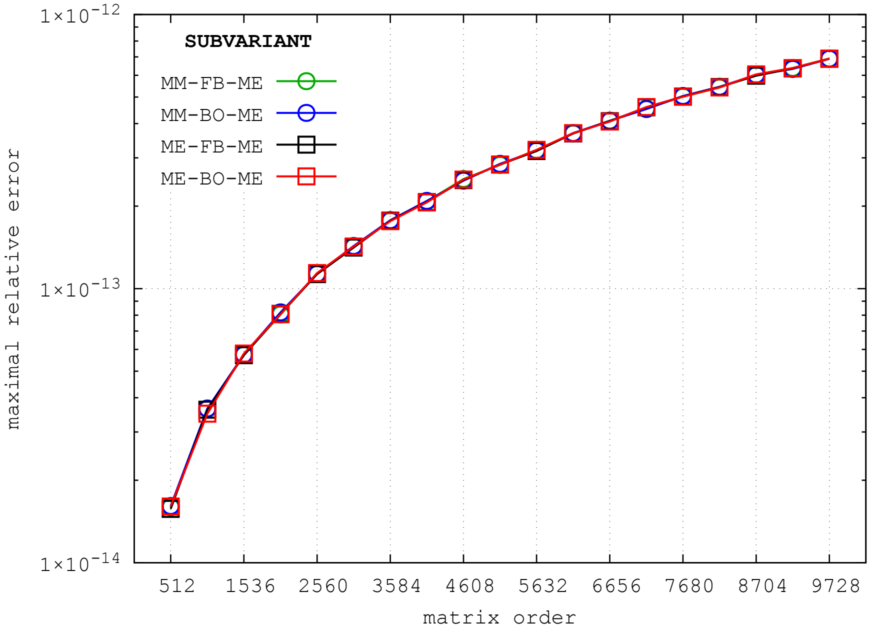


**Figure 83.** The maximal normwise relative error in the computed decomposition of the second matrix in a matrix pair, $\|G - V\Sigma_G X\|_F/\|G\|_F$, for the Algorithm **ZHZ6** on the matrices from the test set, with orders varying from $512$ to $9728$.

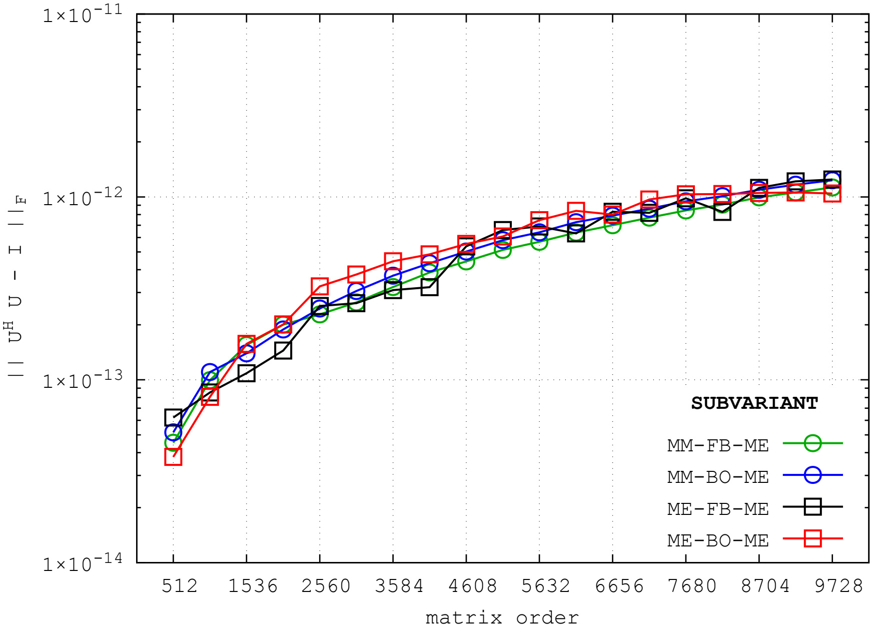


**Figure 84.** Orthogonality $\|U^*U - I\|_F$ of the left generalized singular vectors $U$ for the Algorithm **ZHZ6** on the matrices from the test set, with orders varying from $512$ to $9728$.

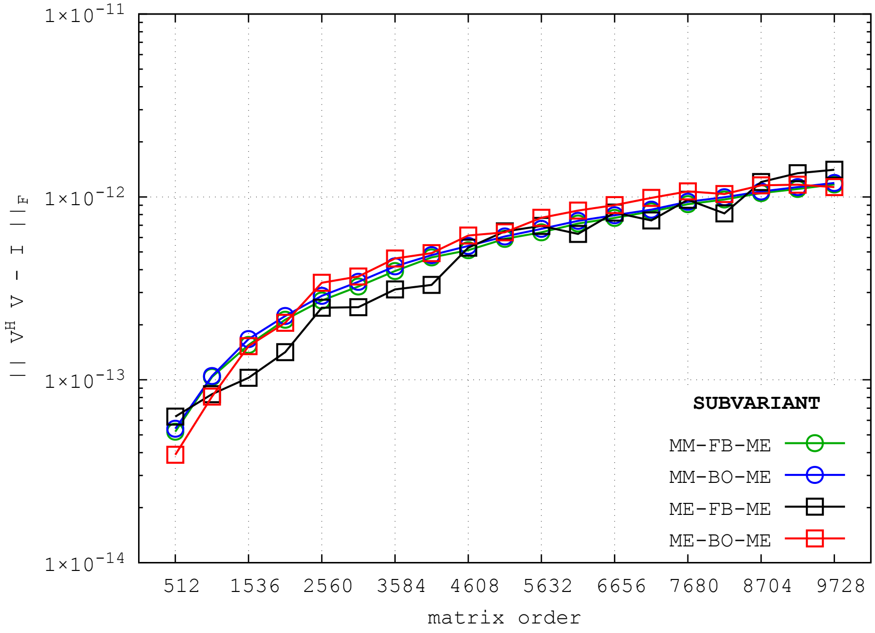


**Figure 85.** Orthogonality $\|V^*V - I\|_F$ of the left generalized singular vectors $V$ for the Algorithm **ZHZ6** on the matrices from the test set, with orders varying from $512$ to $9728$.

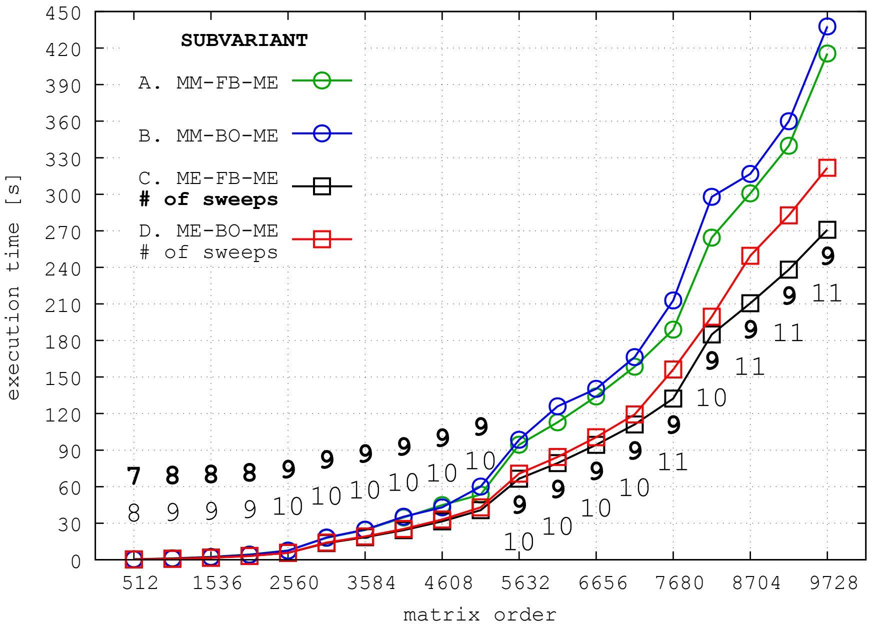


**Figure 86.** The wall execution time and the number of block sweeps for the the block-oriented (BO) and the full block (FB) ZHZ variants, with the outer Jacobi strategies chosen as ME or MM (the inner strategy always being ME), for the Algorithm **ZHZ7** and the matrices from the test set, with orders varying from $512$ to $9728$. The number of sweeps is shown for the ME-BO and the ME-FB (in **bold**). For the MM strategy those numbers are usually larger than for the corresponding ME-using variant.

### *2.2.8 ZHZ7*

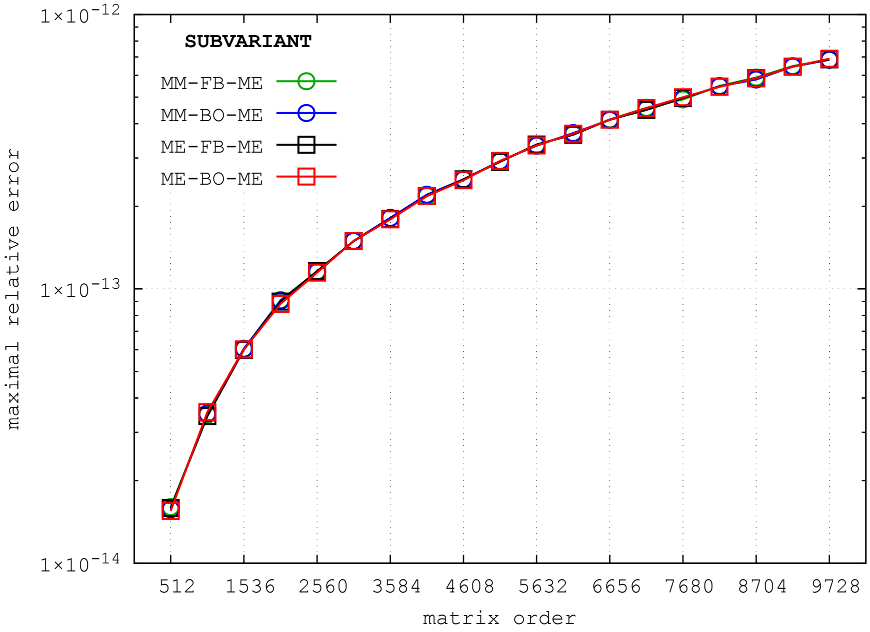


**Figure 87.** The maximal normwise relative error in the computed decomposition of the first matrix in a matrix pair, $\|F - U\Sigma_F X\|_F / \|F\|_F$, for the Algorithm **ZHZ7** on the matrices from the test set, with orders varying from $512$ to $9728$.

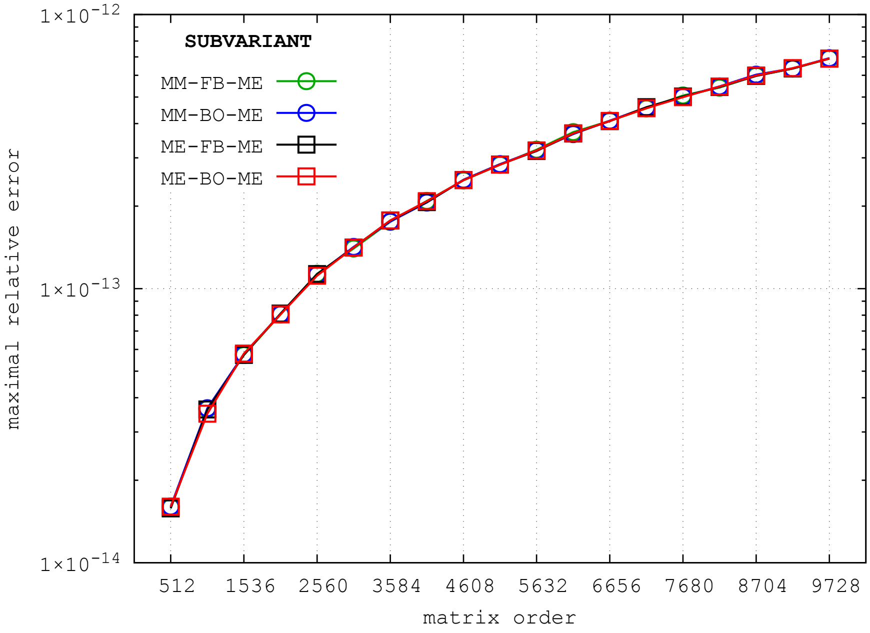


**Figure 88.** The maximal normwise relative error in the computed decomposition of the second matrix in a matrix pair, $\|G - V\Sigma_G X\|_F / \|G\|_F$, for the Algorithm **ZHZ7** on the matrices from the test set, with orders varying from $512$ to $9728$.

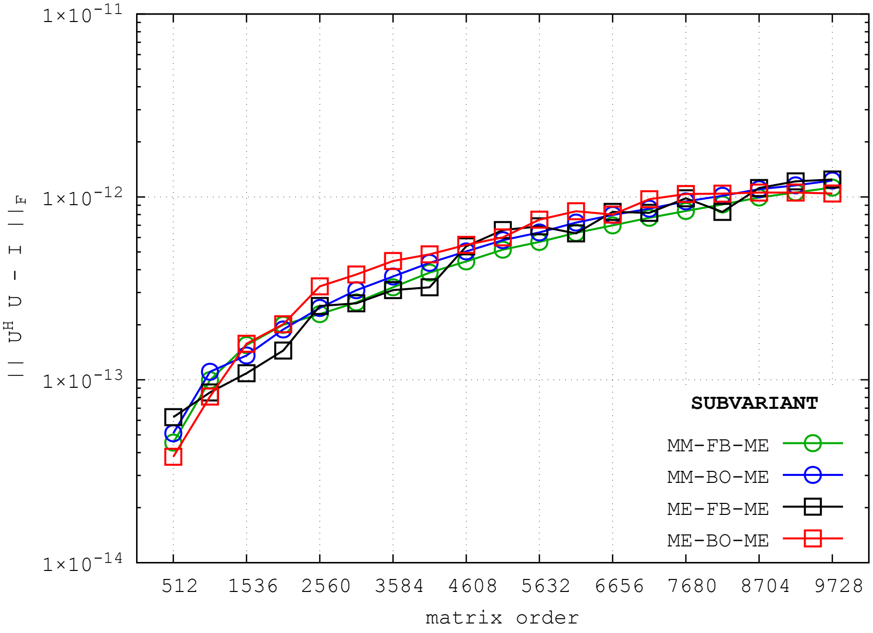


**Figure 89.** Orthogonality $\|U^*U - I\|_F$ of the left generalized singular vectors $U$ for the Algorithm **ZHZ7** on the matrices from the test set, with orders varying from $512$ to $9728$.

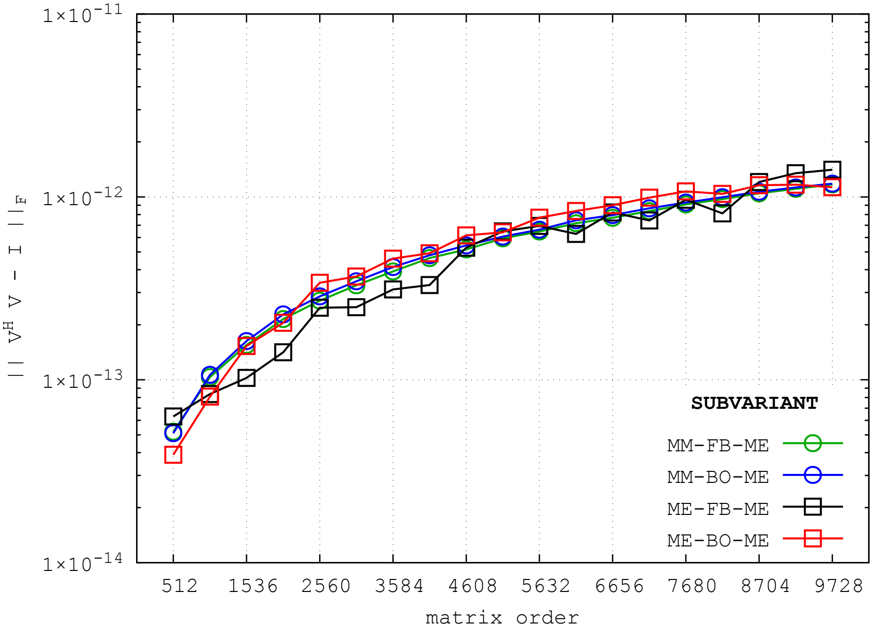


**Figure 90.** Orthogonality $\|V^*V - I\|_F$ of the left generalized singular vectors $V$ for the Algorithm **ZHZ7** on the matrices from the test set, with orders varying from $512$ to $9728$.

## References

Mantharam M and Eberlein PJ (1993) Block recursive algorithm to generate Jacobi–sets. *Parallel Comput.* 19: 481–496. DOI:10.1016/0167-8191(93)90001-2.

Novaković V and Singer S (2011) A GPU-based hyperbolic SVD algorithm. *BIT* 51(4): 1009–1030. DOI: 10.1007/s10543-011-0333-5.

Novaković V, Singer S and Singer S (2015) Blocking and parallelization of the Hari–Zimmermann variant of the Falk–Langemeyer algorithm for the generalized SVD. *Parallel Comput.* 49: 136–152. DOI:10.1016/j.parco.2015.06.004.

## Acknowledgements

This research was performed using the resources of computer cluster Isabella based in SRCE - University of Zagreb University Computing Centre.

## Declaration of conflicting interests

The Authors declare that there is no conflict of interest.

## Funding

This work has been supported in part by Croatian Science Foundation under the project IP–2014–09–3670.
